# Supplementary material for: Unlocking the Wisdom of Large Language Models: An Introduction to The Path to Artificial General Intelligence
Source: arXiv:2409.01007 source file (2025-04-15)
Supplement: Supplementary file 1 [file AppendixB.tex]

\noindent
\begin{table*}[t!]
\begin{small}
\centering
\begin{tabular}{p{0.95\textwidth}}
    \toprule \hline
    \textbf{Sweetheart,} \\
    \\
    Please, please don't be so depressed---We'll be married soon, and then these lonesome nights will be over forever---and until we are, I am loving, loving every tiny minute of the day and night--- \\
    \\
    Maybe you won't understand this, but sometimes when I miss you most, it's hardest to write---and you always know when I make myself---Just the ache of it all---and I can't tell you. If we were together, you'd feel how strong it is---you're so sweet when you're melancholy. I love your sad tenderness---when I've hurt you---That's one of the reasons I could never be sorry for our quarrels---and they bothered you so--- Those dear, dear little fusses, when I always tried so hard to make you kiss and forget--- \\
    \\
    Scott---there's nothing in all the world I want but you---and your precious love---All the material things are nothing. I'd just hate to live a sordid, colorless existence because you'd soon love me less---and less---and I'd do anything---anything---to keep your heart for my own---I don't want to live---I want to love first, and live incidentally... \\
    \\
    Don't---don't ever think of the things you can't give me---You've trusted me with the dearest heart of all---and it's so damn much more than anybody else in all the world has ever had--- \\
    \\
    How can you think deliberately of life without me---If you should die---O Darling---darling Scott---It'd be like going blind...I'd have no purpose in life---just a pretty---decoration. Don't you think I was made for you? I feel like you had me ordered---and I was delivered to you---to be worn---I want you to wear me, like a watch---charm or a button hole bouquet---to the world. \\
    \\
    And then, when we're alone, I want to help---to know that you can't do anything without me... \\
    \\
    All my heart--- \\
    \bottomrule
\end{tabular}
\end{small}
\vspace{-.1in}
\caption{Letter excerpts from Zelda Sayre to F. Scott Fitzgerald \cite{FITZGERALD}}
\label{tab:letter-sample}
\vspace{.1in}
\end{table*}

\section*{Appendix B: Z. Sayre to F. S. Fitzgerald w/ Mixed Emotions}

Analysis of the letter in Table~\ref{tab:letter-sample} shows a complex spectrum of emotions:
\begin{itemize}[leftmargin=1.0em, topsep=-.1em, parsep=-.1em]
\item \textit{Love (+1.0)}: Expressed intensely, especially in phrases like ``there's nothing in all the world I want but you.''
\item \textit{Despair (-1.0)}: Notable in comments like ``I’d have no purpose in life, just a pretty decoration.''
\item \textit{Happiness (+0.6)}: Evident in future plans, ``We’ll be married soon, and then these lonesome nights will be over forever.''
\item \textit{Anxiety (-0.3)}: Shown by ``sometimes when I miss you most, it’s hardest to write.''
\end{itemize}

From the analysis of linguistic behaviors in Chapter~\ref{fig:p1-exp1}, it is evident that a letter can exhibit multiple dominant sentiments. Machine learning methods are equipped with techniques such as feature weighting and entropy analysis to distill these dominant emotions. Unlike human annotators, a machine-learning-trained classifier can consistently produce the same class prediction for a given instance. However, human annotators often show significant variability when identifying dominant sentiments in a letter. For example, if a letter writer's emotions range from ``joyful affective'' to ``longing'' on the sentiment spectrum, different annotators might label it differently—some choosing ``joyful,'' while others opt for ``longing.'' This variability is illustrated in Figure~\ref{fig:pilot2-distributions}. Furthermore, Figure~\ref{fig:pilot2-exp3} demonstrates that all testing letters, except for L\#1, contain more than four sentiments spanning the entire spectrum. This variability may be understandable, considering that love under constraints can evoke tremendous energy of various kinds. Figure~\ref{fig:pilot2-exp4} shows that nearly all letters involve ``joyful'' (11 out of 12) and ``longing'' (9 out of 12) sentiments.

This variability seems to poses challenges in achieving consistent and objective labeling; however, 
the age-old 

leading to inconsistencies in data interpretation and complicating efforts to train and validate linguistic models effectively. To address this issue, it is recommended to identify ground truth by considering a combination of LLM-generated and human-generated labels. This approach aims to harmonize the insights from both human intuition and algorithmic consistency to improve the reliability of sentiment analysis.

\begin{figure*}[t!]
\vspace{-.1in}
    \centering
    \begin{subfigure}[b]{0.45\textwidth}
        \centering
        \vspace{-.07in}
        \resizebox{\linewidth}{150pt}{% Example specific height
            \includegraphics[width=\textwidth]{Chapter10/SemtimentDistrbutionsin12Letters.jpg}
        }
        \vspace{-.15in}
        \caption{\# sentiments in letters }
        \label{fig:pilot2-exp3}
    \end{subfigure}%
    \begin{subfigure}[b]{0.55\textwidth}
        \centering
        \vspace{.03in}
        \resizebox{\linewidth}{150pt}{% Example specific height
            \includegraphics[width=\textwidth]{Chapter10/LettersInSentiment.jpg}
        }
        \vspace{-.15in}
        \caption{\# letters in sentiments}
        \label{fig:pilot2-exp4}
    \end{subfigure}
     \vspace{-.2in}
    \caption{Statistics of Sentiments and Letters}
    \label{fig:pilot2-distributions}
    %\vspace{-.2in}
\end{figure*}
