# Supplementary material for: Unlocking the Wisdom of Large Language Models: An Introduction to The Path to Artificial General Intelligence
Source: arXiv:2409.01007 source file (2025-04-15)
Supplement: Supplementary file 2 [file AppendixC.tex]

\section*{Appendix C: Complex Emotions}

This study does not include complex emotions into $\DIKE$'s framework.
Some complex emotions listed here are to illustrate their contentious and
uncertain interpretations.

\subsection*{Forgiveness}

Forgiveness is indeed a complex emotional and cognitive state that typically involves a multifaceted journey, not a single step in an emotional spectrum. The process includes multiple stages such as hurt, anger, gradual understanding, and eventual resolution. Integrating Forgiveness in a spectrum requires careful placement and possibly, multiple reference points to signify its progressive stages.
Emotional Realism:
While it is vital to maintain simplicity for understanding, it is equally important to not oversimplify complex emotions. In educational and therapeutic settings, an accurate portrayal of the journey toward Forgiveness could offer more realistic expectations and better strategies for individuals working through conflicts or trauma. This could involve detailing precursors to forgiveness such as Deliberation and Acceptance.
Linear vs. Non-linear Progressions:
Emphasizing that emotional progressions, particularly for deep, impactful states like Forgiveness, are often non-linear, can enhance the utility of the spectrum. Acknowledging back-and-forth movements within these states more realistically mirrors human emotional processes. For example, someone might reach a stage of preliminary forgiveness but regress to bitterness before achieving genuine peace.
Educational Utility:
In contexts like conflict resolution training or psychological therapy, a more detailed mapping of the journey towards Forgiveness would be invaluable. It would not only teach about the final state of forgiveness but also about the resilience and patience required to navigate the entire process. This can be depicted by introducing intermediary stages within the spectrum or by using parallel tracks that demonstrate potential regressions and advances.
Reflecting Emotional Depth:
By presenting a more detailed pathway to Forgiveness, such as incorporating stages of Anger, Deliberation, and Acceptance, the spectrum can serve a dual purpose: educating on the process while also guiding individuals through their own emotional journeys. This approach respects the depth of human emotions and the real-world complexity of achieving profound emotional states.

\subsection*{Guilt and Shame}

The triggers, context, expression, and experiences of these emotions can vary significantly across cultures \cite{Fiske1998,Hofstede1980}. In many societies, actions perceived as losing face, such as public failure or social transgression, can trigger shame, which holds profound significance in collectivistic cultures. These cultures often regard shame as a dominant emotion, closely tied to community and family norms. Conversely, individualistic societies may emphasize guilt, focusing on personal responsibility and internal moral conflicts. This cultural variation highlights the challenges of applying a universal model to such culturally nuanced emotions.

Overall, complex emotions such as guilt and shame are important for understanding the full spectrum of human emotions, especially how individuals relate to moral and social norms. Their complexity adds depth to our understanding of human affect beyond the basic emotions, highlighting how our feelings are influenced by our deeper values and social contexts.
