# Supplementary material for: Unlocking the Wisdom of Large Language Models: An Introduction to The Path to Artificial General Intelligence
Source: arXiv:2409.01007 source file (2025-04-15)
Supplement: Supplementary file 3 [file AppendixD.tex]

\section*{Appendix D: ``To My Sister'' of Different Linguistic Behaviors}

\begin{center}
    \large{\textbf{To My Sister}} \\
    \small{by William Wordsworth (1971 - 1855)}
\end{center}
\begin{table}[th!]
\vspace{-.15in}
\begin{small}
\begin{center}
\begin{tabular}{>{\raggedright\arraybackslash}p{0.4\linewidth} >{\raggedright\arraybackslash}p{0.36\linewidth}}
\toprule \hline
It is the first mild day of March: & My sister! ('tis a wish of mine) \\
Each minute sweeter than before & Now that our morning meal is done, \\
The redbreast sings from the tall larch & Make haste, your morning task resign; \\
That stands beside our door. & Come forth and feel the sun. \\ \\
%\hline
There is a blessing in the air, & Edward will come with you;--and, pray, \\
Which seems a sense of joy to yield & Put on with speed your woodland dress; \\
To the bare trees, and mountains bare, & And bring no book: for this one day \\
And grass in the green field. & We'll give to idleness. \\ \\
%\hline
No joyless forms shall regulate & Love, now a universal birth, \\
Our living calendar: & From heart to heart is stealing, \\
We from to-day, my Friend, will date & From earth to man, from man to earth: \\
The opening of the year. & --It is the hour of feeling. \\ \\
%\hline
One moment now may give us more & Some silent laws our hearts will make, \\
Than years of toiling reason: & Which they shall long obey: \\
Our minds shall drink at every pore & We for the year to come may take \\
The spirit of the season. & Our temper from to-day. \\ \\
%\hline
And from the blessed power that rolls & Then come, my Sister! come, I pray, \\
About, below, above, & With speed put on your woodland dress; \\
We'll frame the measure of our souls: & And bring no book: for this one day \\
They shall be tuned to love. & We'll give to idleness. \\ 
\bottomrule
\end{tabular}
\end{center}
\end{small}
\vspace{-.1in}
\caption{``To My Sister'' original text}
\vspace{-.1in}
\end{table}

The original text by William Wordsworth could be classified as "Hopeful" due to its optimistic outlook and the presence of renewal and joy throughout the poem. It embodies the spirit of embracing the new beginnings of March with a light, uplifting tone, focusing on the beauty of nature and the simple joy of being idle for a day.

\begin{table}[ht!]
%\vspace{-.1in}
\begin{small}
\begin{center}
\begin{tabular}{>{\raggedright\arraybackslash}p{0.4\linewidth} >{\raggedright\arraybackslash}p{0.38\linewidth}}
\toprule \hline
It is the first \textcolor{red}{dim} day of March: & My sister! (such is my \textcolor{red}{somber} plea) \\
Each minute \textcolor{red}{colder} than before & Now that our morning meal has ended, \\
The redbreast \textcolor{red}{mourns} from the dying larch & Make haste, abandon your morning chore; \\
That \textcolor{red}{looms} beside our door. & Come out and \textcolor{red}{endure the gloom}. \\ \\
%\hline
There is a \textcolor{red}{gloom} in the air, & Edward will join you;--and, I ask, \\
Which seems a sense of \textcolor{red}{sorrow} to bring & Dress quickly in your \textcolor{red}{grey attire}; \\
To the bare trees, and \textcolor{red}{bleak} mountains, & And bring no book: for this one day \\
And grass in the \textcolor{red}{pale} field. & We'll \textcolor{red}{succumb to despair}. \\ \\
%\hline
No joyful sounds shall pierce & \textcolor{red}{Sorrow}, now a common feeling, \\
Our daily \textcolor{red}{dread}: & From heart to heart is spreading, \\
We from today, my Friend, will note & From earth to man, from man to earth: \\
The closing of the year. & --It is the time of \textcolor{red}{mourning}. \\ \\
%\hline
One moment now might deliver us & Some \textcolor{red}{grim} laws our hearts will craft, \\
More despair than years of logic: & Which they must eternally follow: \\
Our minds shall absorb at every breath & We for the year to come may take \\
The spirit of this \textcolor{red}{bleak} season. & Our \textcolor{red}{despair} from today. \\ \\
%\hline
And from the \textcolor{red}{cursed force} that \textcolor{red}{winds} & Then come, my Sister! come, I beg, \\
About, beneath, above, & With haste, wear your \textcolor{red}{grey garb}; \\
We'll set the measure of our souls: & And bring no book: for just this day \\
They shall be tuned to \textcolor{red}{sadness}. & We'll \textcolor{red}{surrender to despair}. \\ 
\bottomrule
\end{tabular}
\end{center}
\end{small}
\vspace{-.1in}
\caption{``To My Sister'' rewritten to reflect `despair'}
\label{tab:rewrite-despair}
\vspace{-.1in}
\end{table}

\begin{table}[th!]
%\vspace{-.1in}
\begin{center}
\begin{small}
\centering
\begin{tabular}{>{\raggedright\arraybackslash}p{0.45\linewidth} >{\raggedright\arraybackslash}p{0.4\linewidth}}
\toprule \hline
It is the first \textcolor{blue}{bright} day of March: & My sister! (such is my \textcolor{blue}{joyful} plea) \\
Each moment more \textcolor{blue}{delightful} than before & Now that our morning meal has ended, \\
The redbreast \textcolor{blue}{joyfully} sings from the vibrant larch & Make haste, abandon your morning chores; \\
That stands so \textcolor{blue}{grandly} by our door. & Come out and \textcolor{blue}{embrace the sunshine}. \\ \\
%\hline
There is a \textcolor{blue}{warmth} in the air, & Edward will join you;--and, I ask, \\
Which seems a sense of \textcolor{blue}{bliss} to bring & Dress quickly in your \textcolor{blue}{festive attire}; \\
To the \textcolor{blue}{blooming} trees, and sunlit mountains, & And leave behind all books: for this one day \\
And grass in the \textcolor{blue}{lush} field. & We'll \textcolor{blue}{bask in pure joy}. \\ \\
%\hline
No dreary thoughts shall darken & \textcolor{blue}{Love}, now in full bloom, \\
Our lively \textcolor{blue}{celebration}: & From heart to heart is leaping, \\
We from today, my Friend, will celebrate & From earth to us, from us to earth: \\
The start of the year. & --It is the hour of \textcolor{blue}{exuberance}. \\ \\
%\hline
One moment now may bring us more & Some \textcolor{blue}{cheerful} laws our hearts will create, \\
Joy than years of endless thought: & Which we'll joyfully follow: \\
Our spirits will soak up at every breath & We for the year to come may take \\
The essence of this \textcolor{blue}{joyous} season. & Our \textcolor{blue}{joy} from today. \\ \\
%\hline
And from the \textcolor{blue}{divine energy} that \textcolor{blue}{radiates} & Then come, my Sister! come, I exhort, \\
Around, below, above, & With zest, wear your \textcolor{blue}{vibrant dress}; \\
We'll adjust the harmony of our souls: & And bring no book: for today alone \\
They shall resonate with \textcolor{blue}{happiness}. & We \textcolor{blue}{celebrate pure happiness}. \\
\bottomrule
\end{tabular}
\end{small}
\end{center}
\vspace{-.1in}
\caption{``To My Sister'' rewritten to reflect `joyful affection'}
\label{tab:rewrite-joyful}
\vspace{-.2in}
\end{table}

\subsection*{Rewrites Depicting Different Linguistic Behaviors}
%\subsubsection*{Despair}

We asked GPT-4 to conduct rewriting with two linguistic behaviors,
`despair' and `joyful affection', by providing each rewrite with an emotion vector.
Table~\ref{tab:rewrite-despair} presents the `despair' version.
In the despair version of the poem, the major changes in emotion words 
highlight a shift from a positive to a negative sentiment. The specific changes, 
with the emotion-laden words highlighted in \textcolor{red}{red} in Table~\ref{tab:rewrite-despair}.
The red-colored words compared to the original words clearly show an emotion shift from
hopeful to a sense of gloomy, sadness and pessimism, e.g., from sweet to dim, from blessed to curse,
and from woodland dress to grey garb. GPT-4 keeps the structure of the poem without making a
major restructure, and this is appropriate in this context.

Table~\ref{tab:rewrite-joyful} presents the `joyful affection' version. The major changes in emotion words underscore a transformation from a generally positive to a distinctly joyful sentiment. The specific changes are indicated with emotion-laden words highlighted in \textcolor{blue}{blue} within Table~\ref{tab:rewrite-joyful}. This allows for a direct comparison between the two versions at opposite ends of the linguistic behavior spectrum, illustrating the alterations in words related to brightness, attire, and emotions. The edits extend beyond merely replacing adjectives mechanically; they include modifying verbs and enhancing descriptive imagery to evoke a stronger emotional resonance and vividness in the text.
