# Supplementary material for: Unlocking the Wisdom of Large Language Models: An Introduction to The Path to Artificial General Intelligence
Source: arXiv:2409.01007 source file (2025-04-15)
Supplement: Supplementary file 4 [file AppendixE.tex]

\section*{Appendix E: Debate on Modifying Emotional Spectra}

The discussion focuses on proposed modifications to the existing emotional spectra, which aim to introduce more granularity and intricate transitions between emotional states. We critically evaluate the suggestions made by GPT-4, providing refutations for each to ensure that changes preserve the logical progression and clarity of the spectra.

This debate highlights the inherent challenge in finding precise words and placements for emotions within a spectrum. It underscores the importance of establishing a set of commonly agreed-upon emotions as baselines. These baseline emotions serve as anchor points, and the spaces between them can be finely adjusted using scalar factors to represent transitional emotions accurately. This method maintains the integrity of the emotional spectrum and allows for flexibility in depicting a wide range of human emotional experiences.

The emotional journey towards a state, e.g., Forgiveness, often involves various stages, including anger, bitterness, deliberation, and acceptance, which are not captured by simply placing Forgiveness as a midpoint between Composure and Peace. This placement might misrepresent the nature of Forgiveness as being too linear or simplistic, potentially undermining the complexity and the often non-linear process of achieving true forgiveness.

This approach reflects a thoughtful balance between maintaining structured emotional categories and allowing for individual differences and cultural variations in how emotions are experienced and expressed.

\section*{Arguments against Adjustments to the Emotional Spectra}

\subsection*{Terror to Heroism}
\textbf{Suggestion:} Add Anxiety between Fear and Apprehension. \\
\textbf{Refutation:} Anxiety, overlapping significantly with Fear and Apprehension, may not distinctively enrich the spectrum but rather clutter it, diminishing the clarity of emotional transitions.

\subsection*{Grief to Ecstasy}
\textbf{Suggestion:} Include Hope or Optimism between Disappointment and Serenity. \\
\textbf{Refutation:} Introducing Hope or Optimism may disrupt the natural progression from negative to positive emotions, as these emotions imply a leap in emotional recovery that may not sequentially follow Disappointment.

\subsection*{Despair to Elation}
\textbf{Suggestion:} Introduce Relief between Melancholy and Equanimity. \\
\textbf{Refutation:} Relief may better suit transitions associated with specific resolutions of distress rather than being a generic intermediary, potentially disrupting the smooth gradient of the spectrum.

\subsection*{Distrust to Admiration}
\textbf{Suggestion:} Add Gratitude or Appreciation post-Acceptance. \\
\textbf{Refutation:} The emotional journey from Acceptance to Respect inherently encompasses elements of Gratitude and Appreciation, making additional inclusions possibly redundant.

\subsection*{Negligence to Vigilance}
\textbf{Suggestion:} Bridge Interest and Anticipation with Motivation or Determination. \\
\textbf{Refutation:} This addition might complicate the spectrum by implying a volitional shift rather than a gradual increase in attentiveness, which is the main focus of the spectrum.

\subsection*{Rage to Tranquility}
\textbf{Suggestion:} Integrate Forgiveness or Healing to transition from Composure to Peace. \\
\textbf{Refutation:} Forgiveness and Healing, while crucial for achieving tranquility, may not fit well between Composure and Peace, as they could be seen as outcomes of achieving Peace rather than steps towards it.

\subsection*{Loathing to Enthusiasm}
\textbf{Suggestion:} Include Acceptance or Forgiveness between Indifference and Interest. \\
\textbf{Refutation:} These emotions might overcomplicate the transition from aversion to engagement, as they address more specific scenarios rather than general emotional dispositions.

\section*{Defense of the Proposed Adjustments to the Emotional Spectra}

\subsection*{Relevance of Adding Nuanced Emotions}
The introduction of nuanced emotions such as Anxiety between Fear and Apprehension, or Hope between Disappointment and Serenity, is driven by the need for realism in emotional representation, not merely complexity. Emotional experiences are rarely binary; they often involve subtle and complex transitions that are crucial for an accurate depiction of the emotional landscape. These nuances can inform better therapeutic approaches, enhance emotional intelligence training, and provide deeper insights into human behavior, making them essential for realistic portrayals.

\subsection*{Purpose of Including Transitional Emotions}
Inclusion of transitional emotions such as Relief and Gratitude helps bridge the emotional journey from negative to positive states. These emotions act as critical phases in the recovery process, providing a more realistic portrayal of emotional healing. For example, transitioning directly from Melancholy to Equanimity without acknowledging Relief might overlook significant aspects of emotional adjustment.

\subsection*{Utility in Diverse Contexts}
Each proposed emotional state, like Motivation or Determination in the transition from Interest to Anticipation, offers practical insights into how individuals can actively manage their emotional and cognitive states. This understanding is invaluable in educational and professional settings, where knowing how to enhance focus or drive can lead to better outcomes.

\subsection*{Avoiding Oversimplification}
While simplicity in emotional models is valuable, oversimplification can omit critical aspects of emotional experiences. Including emotions such as Forgiveness in the transition from Composure to Peace reflects essential steps in conflict resolution and personal growth. These additions ensure that the spectrum comprehensively addresses managing and resolving intense emotions.

\subsection*{Academic and Practical Implications}
The refined spectrums are designed to cater not only to lay understanding but also to academic and practical applications where depth and precision are crucial. They are particularly useful in fields such as psychology, where an understanding of complex emotional transitions is vital for effective therapy and research.

\subsection*{Conclusion}
The enhancements to the emotional spectra aim to provide a more accurate, realistic, and useful tool for exploring and teaching about emotions. While maintaining clarity and avoiding unnecessary complexity is important, capturing the true richness of human emotional experiences in all their complexity is equally crucial. Therefore, the proposed adjustments are not merely additions but essential elements for depicting a more complete picture of emotional evolution.
