# Supplementary material for: Unlocking the Wisdom of Large Language Models: An Introduction to The Path to Artificial General Intelligence
Source: arXiv:2409.01007 source file (2025-04-15)
Supplement: Supplementary file 6 [file AppendixH.tex]

\section{Appendix H: Instruction to Human Annotators}

As part of the project, we documented the process by which students were involved in annotating a dataset of love letters used for testing.

Students enrolled in my class were asked to
volunteer without pay. 30\% of them responded positively.
They are all US citizens.

They were provided with detailed instructions in class, supplemented by follow-up explanations. The dataset was made available on Google Docs, where students independently rated the letters and submitted their annotations via duplicated spreadsheets. 

The instruction is as follows:

\noindent Dear [Name],

\bigskip

\noindent The attached spreadsheet lists 12 letters collected from the Kaggle Love Letter dataset. Please help annotate these 12 letters with their appropriate linguistic sentiments by following these five steps:

\begin{enumerate}
    \item Duplicate the spreadsheet, and work on your own copy.
    \item \textbf{Read and Understand the Labels:} Make sure you understand each of the seven labels from despair to joyful affection. This will help you accurately categorize the sentiments of each letter.
    \item \textbf{Analyze Each Letter:} Read each letter carefully to understand the predominant emotions. Look for key phrases or words that might indicate a particular sentiment.
    \item \textbf{Assign the Labels:} For each letter, decide which three emotions are most strongly represented. Assign a ``1'' to the most dominant emotion, a ``2'' to the second most dominant, and a ``3'' to the third.
    \begin{itemize}
        \item Despair (extremely negative -1): Indicate profound sadness or hopelessness.
        \item Longing (-0.6): Suggests a strong desire or yearning for someone or something.
        \item Wishful (-0.3): Implies a hopeful desire for something that may or may not be attainable.
        \item Neutral (0): Shows neither positive nor negative emotion; indifferent.
        \item Hopeful (+0.3): Expresses optimism or a looking forward to something positive.
        \item Contentment (+0.6): Reflects a state of satisfaction or peace.
        \item Joyful Affection (extremely positive +1): Denotes a deep joy and love, often vibrant and energetic.
    \end{itemize}
    \item Share with me the completed sheet.
\end{enumerate}

\bigskip

\noindent Thank you so much,

\bigskip

\noindent [My Name]
