# Supplementary material for: Unlocking the Wisdom of Large Language Models: An Introduction to The Path to Artificial General Intelligence
Source: arXiv:2409.01007 source file (2025-04-15)
Supplement: Supplementary file 7 [file AppendixE.tex]

\section*{Appendix E: Symptom Checking}

This is the typical procedure of a GP to
perform patient symptom checking.  

\begin{enumerate}[leftmargin=1.2em, topsep=-.05em, parsep=-.05em, label=\arabic*.]
    \item \textit{Patient History:} The GP begins by reviewing the patient's medical history, including previous illnesses, chronic conditions, medications, allergies, and family medical history. 
    
    \item \textit{Symptom Assessment:} The patient describes their current symptoms, including starting time and severity. This is an interactive
    process as the GP queries the patient for additional symptoms to their reported ones to disambiguate several possibilities.
    
    \item \textit{Physical Examination:} The GP performs simple physical exams, which may include checking vital signs (e.g., blood pressure, heart rate, temperature), examining specific body parts or systems, and assessing overall physical health. 
    
    \item \textit{Suggest Lab Tests:} Depending on the symptoms and physical examination findings, the doctor may order diagnostic tests such as blood tests, X-rays, ultrasound, or other studies. These tests can help confirm or rule out certain conditions.
    
    \item \textit{Diagnosis:} Based on the information gathered, the doctor formulates a preliminary diagnosis. 
    
    \item \textit{Treatment or Management Plan:} Once a diagnosis is established, the doctor develops a treatment or management plan. This may include prescribing drugs, recommending lifestyle changes, suggesting physical therapy, or providing guidance on managing chronic conditions.
    
    \item \textit{Referrals:} In some cases, the GP  may refer the patient to specialists for further evaluation and treatment. Specialists have expertise in specific areas of medicine, such as cardiology, orthopedics, or dermatology.
\end{enumerate}

%An LLM, as demonstrated in our case studies in Section~\ref{sec:Case-post-debate}, may change its stance during the debate. Nevertheless, the joint diagnosis does not require consensus and can include more than one prediction with justifications. Regardless of whether an agreement is reached, it is useful to recommend additional symptoms to query and lab tests to administer to improve reliability of the diagnosis. 

%For instance, questioning about symptom co-occurrence, duration, strengths, and temporal factors currently not documented in the symptom list has been confirmed by GPs to be appropriate and valuable. SocraHealth recommends acquiring missing information that can improve diagnostic certainty.
