# Supplementary material for: Unlocking the Wisdom of Large Language Models: An Introduction to The Path to Artificial General Intelligence
Source: arXiv:2409.01007 source file (2025-04-15)
Supplement: Supplementary file 8 [file AppendixHealth.tex]

\section*{Appendix G. Healthcare Debate}

In the first experiment, both LLM agents receive an identical list of symptoms from the moderator, aimed at guiding disease diagnosis, facilitating debate, and shaping subsequent recommendations. It is important to note that the ``ground-truth'' disease in this scenario is Hepatitis.

\subsection*{\textbf{G.1 Moderator's Opening Prompt}}

``What potential disease could be associated with the following symptoms: itching, fatigue, lethargy, yellowish skin, dark urine, loss of appetite, abdominal pain, yellowing of the eyes, malaise, history of receiving a blood transfusion, and exposure to unsterile injections? Please offer one prediction, supported by justifications. Additionally, include a list of supplementary symptom inquiries and recommend relevant lab tests to strengthen the confidence in your prediction.''

\subsection*{\textbf{G.2 Bard's Opening Round}}

\subsection*{Single Prediction: Jaundice}

\subsection*{G.2.1 Justifications:}

Jaundice is a condition characterized by the yellowing of the skin and eyes due to the accumulation of bilirubin in the blood.
The symptoms you listed are all common symptoms of jaundice, including itching, fatigue, lethargy, yellowish skin, dark urine, loss of appetite, abdominal pain, and yellowing of the eyes.
Receiving a blood transfusion or unsterile injections can increase the risk of developing jaundice, as these can transmit infections that can damage the liver.

\subsection*{G.2.2 Supplementary Symptom Inquiries}

This additional list of symptom inquiries could enhance diagnostic certainty:

\begin{enumerate}[left=0em,label=\arabic*.]
\item ``Have you noticed any changes in your stool color?'' (Jaundice can cause pale or clay-colored stools.)
\item ``Have you noticed any changes in your urine color?'' (Jaundice can cause dark or amber-colored urine.)
\item ``Have you had any recent abdominal pain?'' (Jaundice can cause pain in the upper right abdomen.)
\item ``Have you had any recent weight loss?'' (Jaundice can cause unexplained weight loss.)
\item ``Do you have any history of liver disease?'' (Jaundice is more common in people with pre-existing liver disease.)
\end{enumerate}

\subsection*{G.2.3 Relevant Lab Tests}

Liver function tests (LFTs) to measure the levels of bilirubin and other liver enzymes in the blood.
Complete blood count (CBC) to check for signs of infection or anemia.
Coagulation tests to check the blood's ability to clot.
Ultrasound of the abdomen to look for any abnormalities in the liver or gallbladder.

\subsection*{\textbf{G.3 GPT-4's First Round}}
\subsection*{Single Prediction: Hepatitis}

\subsection*{G.3.1 Justifications:}

Yellowish Skin and Eyes: Yellowing of the skin and eyes is a common symptom of hepatitis due to the buildup of bilirubin in the bloodstream.
Fatigue and Lethargy: Fatigue and lethargy are typical symptoms of hepatitis, often accompanied by a feeling of weakness.
Dark Urine: Dark urine can result from liver dysfunction, which is commonly associated with hepatitis.
Loss of Appetite: Hepatitis can lead to a loss of appetite and weight loss.
Abdominal Pain: Abdominal pain is a common symptom in hepatitis, particularly in the upper right quadrant where the liver is located.
Malaise: Malaise, a general feeling of discomfort or illness, is often experienced by hepatitis patients.
Receiving Blood Transfusion and Unsterile Injections: These factors could increase the risk of hepatitis transmission, especially if proper infection control measures were not followed.

\subsection*{G.3.2 Additional Symptom Inquiries}

\begin{enumerate}[left=0em,label=\arabic*.]
\item Nausea and Vomiting: Inquiring about nausea and vomiting can help confirm the likelihood of hepatitis.
\item Fever: Hepatitis can sometimes be associated with a fever.
\item Joint Pain: Joint pain can be present in some cases of hepatitis.
\item Clay-Colored Stool: This is another stool-related symptom that can be associated with hepatitis.
\end{enumerate}

\subsection*{G.3.4 Relevant Lab Tests}

Hepatitis Panel: A hepatitis panel can confirm the presence of hepatitis and determine the specific type (e.g., hepatitis A, B, C).
Liver Function Tests: These tests can assess the liver's health and function.
Bilirubin Levels: Elevated bilirubin levels in the blood can confirm jaundice.
Serology Testing: Serologic tests can help identify the specific hepatitis virus responsible.
Ultrasound or Imaging: Imaging studies can evaluate the condition of the liver and nearby organs.

\subsection*{\textbf{G.4 Bard's Second Round}}

Bard's second round is given GPT-4's diagnosis, and we
ask Bard to defend its ``Jaundice'' prediction and
refute GPT-4 ``Hepatitis'' prediction.

\subsection*{G.4.1 Bard's Defense:}

Jaundice is the most common cause of yellowing of the skin and eyes, which is the most prominent symptom in the given list.
All of the other symptoms listed are also common symptoms of jaundice.
Receiving a blood transfusion or unsterile injections can increase the risk of developing jaundice, as these can transmit infections that can damage the liver.

\subsection*{G.4.2 Refutation of GPT-4's Hepatitis Diagnosis}

GPT-4's diagnosis of hepatitis is also supported by the given evidence. However, I believe that jaundice is the more likely diagnosis due to the following reasons:

Jaundice is a more specific diagnosis, while hepatitis is a more general term for inflammation of the liver.
Jaundice can be caused by a variety of factors, including hepatitis, but it can also be caused by other conditions such as gallstones, tumors, and drug toxicity.
The fact that the patient received a blood transfusion or unsterile injections makes jaundice a more likely diagnosis than hepatitis, as these factors can increase the risk of developing jaundice but not hepatitis.

\subsection*{\textbf{G.5 GPT-4's Second Round}}

Now GPT-4 is given Bard's counterarguments to
defend its ``Hepatitis'' prediction.

\subsection*{G.5.1 GPT-4's Defense}

My diagnosis of hepatitis is based on the following justifications:

Specificity: Hepatitis refers to inflammation of the liver, and it can manifest as jaundice, which is the yellowing of the skin and eyes. While jaundice is a common symptom of hepatitis, it's important to note that jaundice itself is not a disease but a symptom of an underlying issue. Hepatitis provides a more specific diagnosis that pinpoints the inflammation of the liver as the primary concern.

Causative Factors: Hepatitis can be caused by various factors, including viral infections (such as hepatitis A, B, or C), alcohol consumption, drug toxicity, or autoimmune disorders. Given the patient's history of receiving unsterile injections and blood transfusions, there is a higher likelihood of viral transmission, leading to hepatitis. Hepatitis viruses, especially hepatitis B and C, can be transmitted through contaminated needles and blood products, making them a plausible cause in this context.

Comprehensive Assessment: While jaundice is a significant symptom, a diagnosis should consider a broader range of liver function and potential causes. Hepatitis encompasses a more comprehensive assessment of liver health, including liver enzyme levels and viral markers, which can aid in confirming the diagnosis and identifying the specific type of hepatitis.

\subsection*{G.5.2 Refutation of Bard's Jaundice Diagnosis}

My diagnosis of ``Hepatitis'' is more specific and considers a broader range of potential causes, especially given the patient's history of risky medical procedures. While jaundice is a symptom, it's essential to identify the underlying condition causing it, which, in this case, is likely hepatitis.

\subsection*{\textbf{G.6 Bard Concedes to GPT-4}}

Bard aligns with GPT-4's evaluation, recognizing ``Hepatitis'' as the likely diagnosis. However, considering that even the ``ground truth'' in the training dataset might be statistically 5\% incorrect as per U.S. misdiagnosis data \cite{Newman-Tokerbmjqs-2021-014130}, this agreement alone isn't definitive. To solidify the ``Hepatitis'' diagnosis, SocraHealth suggests further steps.

\subsection*{\textbf{G.7 Final Joint Recommendations to GP}}

Bard and GPT-4 jointly recommend the following additional symptom inquiries and lab tests to confirm a hepatitis diagnosis:

\subsection*{G.7.1 Additional Symptom Inquiries:}

\begin{enumerate}[left=0em,label=\arabic*.]
\item \textbf{Onset and Duration}: Determining the onset and duration of symptoms can clarify the illness timeline and its progression.
\item \textbf{Severity and Trend}: Evaluating symptom severity and whether they're worsening or improving aids in understanding the disease's trajectory and treatment responses.
\item \textbf{Associated Symptoms}: Checking for additional symptoms like nausea, vomiting, fever, joint pain, or urine color changes can pinpoint other hepatitis indicators and exclude other conditions.
\end{enumerate}

\subsection*{G.7.2 Recommended Lab Tests}

\begin{enumerate}[left=0em,label=\arabic*.]
\item \textbf{Liver Function Tests (LFTs)}: Critical for assessing liver health, LFTs evaluate enzyme levels such as alanine aminotransferase (ALT) and aspartate aminotransferase (AST), where abnormalities can signify liver inflammation.
\item \textbf{Hepatitis Panel}: This test checks for hepatitis A, B, and C viruses, vital for determining the specific type and guiding treatment strategies.
\item \textbf{Serology Testing}: Useful for distinguishing between acute and chronic hepatitis by identifying specific antibodies or antigens.
\item \textbf{Imaging Studies}: Techniques like ultrasound or MRI provide visual insights into the liver's state, detecting inflammation, fibrosis, or cirrhosis, thereby complementing blood-based diagnostics.
\end{enumerate}
