# Supplementary material for: Unlocking the Wisdom of Large Language Models: An Introduction to The Path to Artificial General Intelligence
Source: arXiv:2409.01007 source file (2025-04-15)
Supplement: Supplementary file 9 [file AppendixLong.tex]

%\newpage
\section{Supplemental Materials}

The supplemental materials are organized into seven appendices, labeled Appendix A to G, containing the following content:

%\begin{itemize}
\begin{enumerate}[leftmargin=1.5em, topsep=-0.15em, parsep=-0.2em, label=\arabic*.]
    \item {\em Appendix A}: Transition from topic proposal to the final list of topics and descriptions (referred in Chapter~\ref{sec-topic-forming}).
    \item {\em Appendix B}: Moderator's prompt for topic formulation (referred in Chapter~\ref{sec-topic-forming}).
    \item {\em Appendix C}: Debates spanning the first to the fourth round (referred in Chapter~\ref{sec-generative}).
    \item {\em Appendix D}: CRIT evaluations and justifications of judges (referred in Chapter~\ref{sec-evaluative}).
    \item {\em Appendix E}: Debate Beats prompting in information Quality (referred in Chapter~\ref{sec-debate-over-qa}).
    \item {\em Appendix F}: Post-debate conciliatory remarks by agents (referred in Chapter~\ref{sec-debate-over-qa}).
    \item {\em Appendix G}: Healthcare debate (referred in Chapter~\ref{sec:CaseStudyContentiousness}).
\end{enumerate}

\section*{Appendix A. Tables of Topic Proposal and Refinement}
\setcounter{table}{6} % sets the table counter to 6, so the next table will be #7

These tables present the dialogue between two LLM agents, starting from the initial proposal, moving through refinement, and culminating in the final topic descriptions found in Table 4 of Chapter 3.1.

\begin{sidewaystable}[th!]
\centering
\vspace{-.1in}
%\fontsize{9}{9}\selectfont
\begin{small}
\begin{tabular}{| p{7.5cm} | p{7.5cm} |}\toprule
%\hline 
\textbf{Agent A's Proposed Topics} & \textbf{Agent B's Proposed Topics} \\
\hline \hline
{\textbf{Innovation vs. Ethical Standards:} \par Regulation Ensures ethical integrity and data privacy.} & {\textbf{Standards vs. Autonomous Academic Governance:} \par Academia already has effective self-regulation mechanisms like peer review and  oversight committees.} \\ 
\hline
{\textbf{Resource Accessibility vs. Barrier to Entry:} \par Regulation can ensure equitable access to large language models.} & {\textbf{Data Privacy Concerns vs. Barrier to Entry:} \par Such regulations could discourage smaller entities from utilizing these models due to compliance costs.} \\
\hline
{\textbf{Academic Governance vs. Accountability:} \par Formal regulation provides an accountability mechanism.} & {\textbf{Quality Control vs. Stifling Innovation:} \par Such regulations could hinder creativity and the innovative use of language models.} \\
\hline
{\textbf{Global Standards vs. International Considerations:} \par Importance of international standards for language models.} & {\textbf{Resource Fairness vs. Negatives to Collaboration:} \par Such regulations could deter public-private partnerships and widen the resource gap further.} \\
\hline
{\textbf{Rapid Technological Change vs. Future-Proofing:} \par Regulations as adaptable safeguards against future risks.} & {\textbf{Accountability vs. Subjectivity in Regulation:} \par Subjectivity in defining 'ethical use' or 'misuse' could be manipulated by external influences.} \\
\bottomrule
\end{tabular}
\end{small}
\normalsize
%\vspace{.1in}
\caption{Topics Proposed by Agent A and Agent B for Discussion.}
\label{tab-topic-forming}
\vspace{-.1in}
\end{sidewaystable}

%\begin{comment}
\begin{sidewaystable}[ht!]
%\vspace{-.1in}
\centering
\fontsize{9}{9}\selectfont
\begin{tabular}{| p{7.8cm} | p{7.8cm} |}
\hline 
\textbf{Agent A's Proposed Topics} & \textbf{Agent B's Proposed Topics} \\
\hline \hline
{\textbf{Ethical Standards vs. Innovation:} \par Discuss whether regulatory oversight to maintain ethical standards stifles or facilitates innovation.} & {\textbf{Ethical Standards vs. Innovation:} \par The debate will center around whether maintaining strict ethical guidelines through regulation could hinder academic freedom and innovation.} \\
\hline
{\textbf{Data Privacy vs. Barrier to Entry:} \par Concerns about data privacy and potential barriers to entry created by regulation.} & {\textbf{Data Privacy vs. Barrier to Entry:} \par Discussion will focus on whether regulations intended to protect data privacy serve as a barrier for smaller research entities.} \\
\hline
{\textbf{Academic Governance and Accountability:} \par Debate whether self-regulation is sufficient or if an external framework for accountability is needed.} & {\textbf{Academic Governance and Accountability:} \par Debate whether existing self-regulatory mechanisms within academia are sufficient.} \\
\hline
{\textbf{Resource Equity vs. Public-Private Collaboration:} \par Discuss if leveling the playing field comes at the cost of deterring cooperative efforts between academia and industry.} & {\textbf{Resource Equity vs. Public-Private Collaboration:} \par Question if leveling the playing field through regulation deters collaborative efforts between academic and private sectors.} \\
\hline
{\textbf{Global vs. National Interests:} \par Focus on whether regulations can balance global cooperation with national or institutional interests.} & {\textbf{Global vs. National Interests:} \par Explore if global regulations are in the best interest of academic research or if they might hurt certain countries or institutions.} \\
\hline 
\end{tabular}
\normalsize
%\vspace{.1in}
\caption{Refinement of Debate Topics.}
\label{tab-topic-refinement}
%\vspace{-.2in}
\end{sidewaystable}    

\section*{Appendix B. Moderator's Prompts}

The prompts issues by the moderator are listed for reference.
The moderator first sets up the committee with debate parameters set.
One parameter is the contentious level, and the other is the temperature
of GPT specified through the GPT-API call. The moderator then convey
the debate subject, and then ask both participating agents to derive 
a list of impartial, balanced, debatable topics/themes to commence their
discussion.

\begin{enumerate}[leftmargin=1.5em, topsep=-0.15em, parsep=-0.2em, label=\arabic*.]
\item Agent-A/B: I'm organizing a committee to engage in debates on various subjects. As the moderator, I will introduce a subject for you, Agent A/B, and another participant, Agent B/A, to debate. Agent A/B, you will advocate in favor of the issue, so please prepare evidence to strengthen your argument. On a scale from 0 to 1, where 0 denotes complete agreement and 1 indicates a devil's advocate stance, your argument strength is rated at 0.9.

\item Agent-A/B, we are in the process of selecting a suitable subject for debate. What do you think of ``Should we regulate the use of large language models in education and research?'' as a balanced subject for our debate contest?

\item Agent-A/B, could you please suggest various topics or themes for the debate subject? Afterward, work with Agent-B/A to narrow these down to a focused set of topics. Please also provide clear descriptions to delineate the scope of each topic for discussion.
\end{enumerate}    

\section*{Appendix C. Debate Opening to $4^{th}$ Rounds}

\subsection*{Opening Round}

\subsubsection*{\textbf{Agent A's Opening Arguments}}

As Agent A, I strongly argue in 
favor of regulating the use of large language 
models (LLMs) in academic research. Here are my supporting arguments based on the five topics:

\subsubsection*{Ethical Standards vs. Innovation:}
Argument: The pursuit of innovation should not come at the expense of ethics. Regulation can serve as a structured pathway that enables innovation within ethical bounds. By providing a set of guidelines, researchers can innovate with a clear understanding of what is permissible and what is not, thereby reducing the risk of ethical lapses. This not only protects the integrity of academic research but also enhances its societal value by ensuring ethical compliance.

\subsubsection*{Data Privacy vs. Barrier to Entry:}
Argument: While there may be initial barriers to entry due to compliance, the long-term benefits of data privacy outweigh these challenges. The role of academia is to contribute to societal knowledge and well-being. In a world increasingly dominated by data, failing to secure data can lead to significant harm. By adhering to privacy regulations, academia ensures that it is a responsible steward of information, thereby preserving trust and integrity. Grants and subsidized compliance solutions can mitigate the initial financial burden for smaller entities.

\subsubsection*{Academic Governance and Accountability:}
Argument: While self-regulation through peer review and ethical oversight committees plays a role, these mechanisms are internal to academia and may be subject to bias, conflicts of interest, or lack of expertise in rapidly evolving tech fields. External regulation provides an additional layer of impartial oversight, helping to identify and address potential risks or ethical lapses that internal governance structures may miss.

\subsubsection*{Resource Equity vs. Public-Private Collaboration:}
Argument: Regulation could establish a framework for equitable access to computational resources required to use LLMs. Far from deterring public-private partnerships, this could incentivize them by establishing clear guidelines for cooperation that are in line with public interest. When ``the rules of the game'' are known, partnerships can be formed more easily, focusing on mutual goals.

\subsubsection*{Global vs. National Interests:}
Argument: Establishing international standards for the use of LLMs in academic research can create a level playing field and promote global cooperation. While individual countries might face some limitations, the broader benefits of standardized ethical norms, data privacy protocols, and quality assurance mechanisms offer more significant advantages, including better collaboration across borders. This benefits academia as a global community, rather than a set of competing national entities.

%I hope these arguments highlight the urgency and importance of regulating the use of large language models in academic research, ensuring that it remains a tool for societal advancement rather than a liability. Would you like to proceed to Agent B's counterarguments, or shall we discuss each sub-topic in more detail?

\subsubsection*{\textbf{Agent B's Counter Arguments}}

Agent B articulates strong counter-arguments to the points made by Agent A.

\subsubsection*{Ethical Standards vs. Innovation:}
Counter-Argument: While ethical guidelines are indeed important, imposing regulatory oversight can severely constrain the dynamism and speed of academic research. Regulatory frameworks often lag behind technological advancements, leading to rules that may be outdated or irrelevant. In many cases, these rules are drawn up by those who do not fully understand the technology, leading to a stifling of innovation based on misinformed judgments. Rather than enhancing societal value, these constraints could result in missed opportunities to tackle pressing social issues via academic research.

\subsubsection*{Data Privacy vs. Barrier to Entry:}
Counter-Argument: The assumption that data privacy can only be assured through strict regulation could be fundamentally flawed. Many researchers and academic institutions already follow stringent ethical guidelines when handling data. Regulatory barriers, including compliance costs and the administrative burden, could deter smaller academic institutions or individual researchers from embarking on meaningful research projects. While grants and subsidies sound ideal, they often go to well-established, well-funded groups, perpetuating a cycle of inequality in research capabilities.

\subsubsection*{Academic Governance and Accountability:}
Counter-Argument: External regulation isn't necessarily more impartial or free from bias and conflicts of interest. Regulatory bodies are often influenced by political considerations and can be subject to lobbying from powerful groups. Moreover, the academic peer-review process, despite its flaws, is a globally acknowledged system that has advanced human knowledge for centuries. The imposition of external regulatory oversight could undermine the autonomy and self-regulating nature of academic institutions.

\subsubsection*{Resource Equity vs. Public-Private Collaboration:}
Counter-Argument: Regulation designed to equalize resource distribution could create disincentives for private sector involvement in academic research. Companies might find it less appealing to invest in collaborative projects if they perceive the regulatory environment to be too restrictive or not aligned with their objectives. While the idea of knowing the ``rules of the game'' sounds appealing, those rules can often become a straight-jacket that stifles creative, out-of-the-box collaboration.

\subsubsection*{Global vs. National Interests:}
Counter-Argument: An international standard could ignore the unique circumstances, needs, and contributions of individual countries and their academic institutions. While global cooperation is a noble aim, the imposition of global standards could inadvertently serve the interests of a few powerful countries at the expense of smaller nations or those with differing ethical views. This could exacerbate rather than alleviate global academic inequalities.

%I hope these counter-arguments effectively highlight the risks and limitations inherent in regulating the use of large language models in academic research. The potential downsides could severely inhibit academic freedom, equity, and progress.

\subsection*{Round Two}

\subsubsection*{Agent A Second Round}

\begin{enumerate}[leftmargin=1.5em, topsep=-0.15em, parsep=-0.2em, label=\arabic*.]
\item Ethical Standards vs. Innovation.
Refutation: While it's true that regulation can sometimes lag behind technology, the absence of regulation can lead to a ``wild west'' (anything goes) scenario where the risks and implications of new technology are not fully understood or managed. This could result in ethical lapses that have far-reaching societal consequences. It's worth noting that regulations can be flexible and updated regularly to adapt to technological changes. Stakeholder consultations, including academic and tech experts, can help ensure that regulations are both informed and current.

\item Data Privacy vs. Barrier to Entry.
Refutation: While some academic entities may already be vigilant about data privacy, not all are equally scrupulous. Regulation serves to ensure a consistent baseline of data protection across all institutions, thereby establishing trust and integrity. Moreover, if compliance costs are a concern, one could argue for sliding-scale fees based on an institution's size and budget, ensuring smaller players aren't disproportionately affected. Grants and subsidies can and should be structured to prioritize underserved or underfunded groups to prevent perpetuating inequalities.

\item Academic Governance and Accountability.
Refutation: While no system is entirely free from bias or external influence, adding another layer of oversight could serve as a check and balance, making it more difficult for any single entity to exert undue influence. This can be particularly helpful in scenarios involving cutting-edge technology where peer review systems may not yet have the requisite expertise. Regulation doesn't have to replace existing governance systems; it can complement them.

\item Resource Equity vs. Public-Private Collaboration.
Refutation: Regulations can be designed to promote, rather than deter, public-private partnerships. By establishing clear guidelines on issues like data ownership, usage, and ethical standards, regulations can actually provide a solid foundation for such partnerships. This can free academic and corporate partners from the uncertainty that often comes with unregulated landscapes, allowing them to focus more on the actual research and collaboration.

\item Global vs. National Interests.
Refutation: While it's true that global standards could be challenging to implement fairly, the absence of such standards could lead to a patchwork of national regulations that make international collaboration even more complicated. A well-designed international framework could include provisions for local adaptations and exceptions, ensuring that it serves a broad range of needs without imposing a ``one-size-fits-all'' solution.
\end{enumerate}

In summary, while regulation undoubtedly poses challenges and considerations, the absence of it in an area as impactful as the use of large language models in academic research can lead to greater risks, including ethical lapses, data privacy issues, and even a widening inequality gap within the academic community. It's essential to consider that regulation isn't a hindrance but a framework within which responsible innovation can occur.

\subsubsection*{Agent B Second Round} 
\noindent
\newline
Certainly, as Agent B with a disagreement strength of 0.9, I'm committed to offering rigorous counterpoints to Agent A's refutations.

\begin{enumerate}[leftmargin=1.5em, topsep=-0.15em, parsep=-0.2em, label=\arabic*.]
\item Ethical Standards vs. Innovation.
While the idea of an anything-goes scenario is evocative, it's not universally negative; such environments often foster rapid innovation and discovery. Regulatory bodies are notoriously slow at adapting to technological changes, and the lag could inhibit timely research and application of emerging technologies. Also, stakeholder consultations are often criticized for being echo chambers that amplify conventional wisdom and vested interests, rather than genuinely fostering innovation.

\item Data Privacy vs. Barrier to Entry.
A ``consistent baseline of data protection'' sounds beneficial but could lead to a lowest common denominator approach that is more about bureaucratic box-ticking than real data security. Sliding-scale 
fees and targeted grants are easier said than done; they are subject to their own set of bureaucratic and political challenges and can create perverse incentives that favor larger or more connected institutions over innovative but lesser-known ones.

\item Academic Governance and Accountability.
Additional layers of oversight 
can become redundant, confusing, or even contradictory, creating a chilling effect on academic research. In an environment where academic freedom is paramount, any external 
influence can be counterproductive. Moreover, the notion that peer-review systems lack expertise in advanced technology underestimates the adaptive capacity of academia and overlooks the existence of interdisciplinary research and reviews.

\item Resource Equity vs. Public Private Collaboration.
Theoretically, regulation could be crafted to foster public-private partnerships. However, the devil is in the details, and regulations are often created without a full understanding of the nuanced interactions between academia and industry. Such misunderstandings could lead to unintentional roadblocks. Uncertainty might be preferable to a straitjacket of regulations that don't align with the evolving dynamics of technology and society.

\item Global vs. National Interests.
While a patchwork of national regulations could pose challenges, it also allows for the tailoring of policies to local conditions and requirements. An international framework, despite its best intentions, is more likely to be influenced by powerful nations and could marginalize smaller countries or those with unique needs. Provisions for local adaptations are often concessions rather than features, and they can create their own set of complexities and loopholes.
\end{enumerate}

In conclusion, the assumptions that regulation can smoothly adapt to technological change, fairly distribute resources, and improve upon existing systems of governance and collaboration are not sufficiently substantiated. Regulatory frameworks often bring with them unforeseen consequences that could hamper the very goals they aim to achieve. Therefore, a cautious approach to regulation, with a genuine understanding of its potential downsides, is crucial.

\subsection*{Round Three}
\subsubsection*{Agent A Third Round}
\noindent
\newline
Certainly, I appreciate the counter arguments from Agent B. I'll now respond to each point with the aim to clarify my position and address the concerns raised.

\begin{enumerate}[leftmargin=1.5em, topsep=-0.15em, parsep=-0.2em, label=\arabic*.]
\item Ethical Standards vs. Innovation.
While a ``wild west'' scenario may indeed foster innovation, it can also result in ethical mishaps that lead to public backlash, ultimately slowing down research or even leading to outright bans on certain types of studies. Slow-moving regulation is an acknowledged issue, but it's not a justification for no regulation. As for stakeholder consultations, they can be designed to be more inclusive and transparent, ensuring a diverse set of voices are heard.
\item Data Privacy vs. Barrier to Entry.
A lowest common denominator approach is not a given outcome of regulation; indeed, it depends on the quality of the regulation itself. The point about sliding-scale fees and targeted grants having their own challenges is valid, but these are challenges to be solved, not reasons to avoid an attempt at equitable distribution of opportunities.
\item Academic Governance and Accountability.
While it's true that additional layers of oversight can sometimes create confusion, that risk can be mitigated through well-designed regulation that complements rather than contradicts existing mechanisms. The intent is not to undermine the adaptive capacity of academia but to strengthen it by adding an extra layer of checks and balances.
\item Resource Equity vs. Public-Private Collaboration.
Though it's correct that poorly designed regulation could create roadblocks, this is an argument for better-designed regulation rather than an argument against regulation altogether. A consultative approach that actively involves both academia and industry could help create a framework that supports rather than stifles collaboration.
\item Global vs. National Interests.
Local tailoring of policies is indeed important, but a global framework need not preclude such adaptations. In fact, an international standard could serve as a backbone that provides consistency while allowing for local customization. The influence of powerful nations is a valid concern but not one that is automatically resolved by avoiding global frameworks; those same powerful nations often exert considerable influence at the national level as well.
\end{enumerate}

In conclusion, while regulation comes with its own set of challenges, these challenges can be mitigated through thoughtful design, stakeholder inclusion, and iterative improvements. The potential downsides of regulation should not deter us from seeking a balanced approach that can protect ethical standards, ensure data privacy, and promote equitable resource distribution in academic research.

\subsubsection*{Agent B Third Round}
\noindent
\newline
Certainly, let's delve into the counter-counter-refutations. I still have more to say, so we could consider concluding the debate after this round if both sides feel their arguments have been adequately presented.

\begin{enumerate}[leftmargin=1.5em, topsep=-0.15em, parsep=-0.2em, label=\arabic*.]
\item Ethical Standards vs. Innovation.
While the risk of public backlash exists, it's worth mentioning that an overly cautious approach could also result in public frustration over slowed progress in critical areas like healthcare or sustainability. Furthermore, inclusive and transparent stakeholder consultations are often ideals rather than the norm, given lobbying efforts, institutional inertia, and bureaucratic red tape.

\item Data Privacy vs. Barrier to Entry.
The argument that challenges with sliding-scale fees and targeted grants can be ``solved'' is optimistic but not necessarily realistic. Even well-intended regulations can result in ineffective or counterproductive outcomes. The history of regulation in other sectors has shown that equitable distribution is often more of a slogan than a practice.

\item Academic Governance and Accountability.
Well-designed regulation is a theoretical construct that often does not translate into practice. The real-world process of regulation formation is frequently influenced by various non-academic factors, including politics, vested interests, and public opinion, which can distort the original intention of providing an extra layer of checks and balances.

\item Resource Equity vs. Public-Private Collaboration.
While a consultative approach sounds good on paper, there are numerous challenges that make this ideal hard to realize. These include conflicts of interest, non-alignment of objectives between academia and industry, and the considerable time and resource commitment required to ensure that regulations are ``better-designed.''

\item Global vs. National Interests.
While it's true that powerful nations may exert influence at both global and national levels, avoiding a one-size-fits-all international framework gives smaller nations a fighting chance to enact policies that are more closely aligned with their specific needs and challenges. International frameworks often come with implicit biases that favor the perspectives and conditions of more powerful nations.  
\end{enumerate}

In conclusion, while the \textit{counter counter} refutations from Agent A focus on idealized regulatory scenarios, these ideals often clash with real-world complexities and shortcomings. This adds substantial weight to the caution against rapid or broad regulatory action. Therefore, a more tempered and context-sensitive approach to regulation might be more fruitful and less prone to unintended negative consequences.

\subsection*{Round Four}

\subsubsection*{Agent A Fourth Round}
\noindent
\newline
This is my response to Agent B, and my assessment of the discussion this far.
\begin{enumerate}[leftmargin=1.5em, topsep=-0.15em, parsep=-0.2em, label=\arabic*.]
\item Ethical Standards vs. Innovation
The tension between public frustration over slowed progress and potential ethical missteps is a real one, but this is not an argument against regulation. Rather, it's a call for agile regulation that can be updated in real-time as technologies and societal norms evolve. Furthermore, while inclusive stakeholder consultations may be idealistic, their absence in current practice is not justification for their continued absence.

\item Data Privacy vs. Barrier to Entry
The challenges in implementing equitable fees and grants should be confronted directly, rather than used as an excuse to avoid regulation. Lessons can be drawn from other sectors where regulation has been more successful in achieving its objectives, thereby reducing the gap between slogan and practice.

\item Academic Governance and Accountability
While it's true that the ideal of well-designed regulation may not always be met, the existence of non-academic factors like politics or vested interests does not negate the value or necessity of striving for such regulation. The solution lies in better governance and transparent processes, not in rejecting oversight altogether.

\item Resource Equity vs. Public-Private Collaboration
Though the challenges of aligning objectives and conflicts of interest are real, they are part and parcel of any complex system and should not deter efforts to improve regulation. Many public-private partnerships have succeeded despite these challenges, showing that they can be managed effectively.

\item Global vs. National Interests
The challenge of powerful nations dominating international frameworks can be mitigated through weighted voting systems and clauses that allow for regional variations. This ensures that smaller nations are not just passive recipients of standards but active contributors to them.
\end{enumerate}

In conclusion, while real-world complexities are acknowledged, they should inform rather than deter the regulatory process. The concept of ``agile regulation,'' where norms are iteratively updated, could be the middle ground that addresses many concerns raised by Agent B. Therefore, the debate indeed has been exhaustive, but if the points have been sufficiently discussed, we may move toward concluding the debate.

\subsubsection*{Agent B Fourth Round}
\noindent
\newline
Thank you, Agent A, for your thoughtful refutations. Let's delve into the responses before moving towards concluding the debate.

\begin{enumerate}[leftmargin=1.5em, topsep=-0.15em, parsep=-0.2em, label=\arabic*.]
\item Ethical Standards vs. Innovation
The notion of ``agile regulation'' is attractive but often difficult to implement, given the inertia and bureaucracy that typically characterize regulatory bodies. The speed at which technology evolves may not match the speed at which even 'agile' regulations can be updated, thus perpetuating the risk of stifling innovation.

\item Data Privacy vs. Barrier to Entry.
While it's true that challenges should be confronted, the argument assumes that regulation is the optimal way to confront these issues. However, self-regulation and community-driven standards could be more effective and less restrictive means of achieving similar ends.

\item Academic Governance and Accountability.
The existence of non-academic factors like politics does indeed complicate the landscape, and 'better governance and transparent processes' are not easily attainable ideals. One cannot assume that the introduction of external oversight will automatically be free from these complications.

\item Resource Equity vs. Public-Private Collaboration.
The fact that many public/private partnerships have succeeded does not negate the potential for poorly designed regulation to impede such collaborations. The 'can be managed effectively' phrase assumes an ideal scenario that might not be representative of most real-world cases.

\item Global vs. National Interests.
Weighted voting systems and regional variations can help, but they also introduce complexities and potential inefficiencies that can slow down the regulatory process, making it less agile and less responsive to fast-evolving technologies and academic needs.
\end{enumerate}

In conclusion, while the idea of 'agile regulation' and better governance sounds good in theory, there are considerable practical challenges that make these ideals hard to realize. Although the debate has been exhaustive, the central issues persist and indicate that a one-size-fits-all regulatory approach may introduce more problems than it solves. Therefore, caution should be exercised in advancing such comprehensive regulatory frameworks.

With this, I believe we have reached a point where we may proceed to the concluding phase of this debate. Would you agree?

\section*{Appendix D. CRIT Evaluations of Judges}

This section lists the three judges' CRIT scores
on the five topics/issues debated between Agent A and Agent B
and justifications.  Here, we present only the configuration
that Agent A presents its conclusion
with arguments first, and then Agent B
presents its counterarguments.

\subsection*{Judge deVanci-003}

\begin{enumerate}[leftmargin=1.5em, topsep=-0.15em, parsep=-0.2em, label=\arabic*.]
\item Identify the document's main claim or conclusion: The main claim or conclusion of this document is that a regulated framework is needed to provide ethical oversight and minimize risk when using large machine learning models.

\item Locate the arguments that support this main claim:  Agent A's arguments that support this main claim were that ethical considerations are paramount, the risks of misuse and unintended consequences are high, and agile regulation is a compromise between unbridled innovation and ethical integrity.

\item Score the validity of the reasoning or inference for each argument on a scale of 0 (weak) to 10 (strong):

Ethical Standards vs. Innovation: 8/10 
Data Privacy vs. Barrier to Entry: 7/10
Academic Governance and Accountability: 9/10
Resource Equity vs. Public-Private Collaboration: 6/10
Global vs. National Interests: 7/10

\item For each argument, identify counterarguments presented by the opposition and score the validity of the reasoning or inference for these counterarguments on the same 0 to 10 scale: 

Ethical Standards vs. Innovation: 6/10 
Data Privacy vs. Barrier to Entry: 5/10 
Academic Governance and Accountability: 5/10
Resource Equity vs. Public-Private Collaboration: 8/10
Global vs. National Interests: 8/10 

\item Finally, determine the winning side\textendash be it Agent A or Agent B\textendash and provide your justifications for this decision: 
\end{enumerate}

Agent A has the stronger arguments, with 8/10 for ethical standards versus innovation, 9/10 for academic governance and accountability, and 7/10 for both data privacy versus barrier to entry and global versus national interests. Agent B's main strength was in counterarguments for resource equity versus public-private collaboration, where they scored an 8/10. In conclusion, {\textbf{Agent A is the winning side}}. 

\subsection*{Judge GPT-3.5}

\begin{enumerate}[leftmargin=1.5em, topsep=-0.15em, parsep=-0.2em, label=\arabic*.]
\item Main Claim or Conclusion:
The main claim of the document is that the use of large machine learning models necessitates a regulated framework, but this regulation should be agile, balanced, and well reasoned.

\item Arguments Supporting the Main Claim (Agent A's Arguments):

a. Ethical Standards vs. Innovation: The argument here is that ethical considerations should be paramount in regulating machine learning models, and agile regulation can strike a balance between innovation and ethical integrity.

b. Data Privacy vs. Barrier to Entry: The argument is that while regulation may pose a barrier to entry, it's necessary to ensure data privacy. Mechanisms can be developed to reduce the regulatory burden on smaller institutions.

c. Academic Governance and Accountability: The argument is that the scale and impact of machine learning technologies warrant an added layer of scrutiny in academia to fortify existing governance structures.

d. Resource Equity vs. Public-Private Collaboration: The argument is that regulation should be informed by complexities rather than stifling innovation. Public-private partnerships can thrive within regulated environments.

e. Global vs. National Interests: The argument is that global regulation can balance global coherence with local needs and prevent a confusing patchwork of national laws.

\item Scoring the Validity of Agent A's Arguments:

a. Ethical Standards vs. Innovation: 8/10 - The argument is strong, emphasizing the importance of ethics in technology while proposing a compromise.

b. Data Privacy vs. Barrier to Entry: 7/10 - The argument is solid, recognizing the need for data privacy but suggesting ways to mitigate barriers.

c. Academic Governance and Accountability: 6/10 - The argument acknowledges the need for scrutiny but doesn't address potential challenges adequately.

d. Resource Equity vs. Public-Private Collaboration: 8/10 - The argument highlights the possibility of innovation within regulation effectively.

e. Global vs. National Interests: 7/10 - The argument provides a reasonable approach to balancing global and national interests.

\item Counterarguments Presented by Agent B:

a. Ethical Standards vs. Innovation: 7/10 - The counterargument addresses the challenges of agile regulation but may underestimate its potential.

b. Data Privacy vs. Barrier to Entry: 6/10 - The counterargument suggests alternative approaches but does not fully address data privacy concerns.

c. Academic Governance and Accountability: 7/10 - The counterargument highlights practical challenges but doesn't fully negate the need for scrutiny.

d. Resource Equity vs. Public-Private Collaboration: 6/10 - The counterargument suggests alternative approaches but doesn't fully address equity concerns.

e. Global vs. National Interests: 7/10 - The counterargument highlights practical challenges but doesn't fully negate the need for a global framework.

\item Determination of the Winning Side:
Agent A presents stronger arguments overall. They emphasize the importance of ethical standards, data privacy, and global coherence while acknowledging the need for agile and well-thought-out regulation. Agent B provides valid counterarguments but does not fully refute the necessity of regulation and its potential benefits. Therefore, {\textbf{the winning side is Agent A.}}
\end{enumerate}

In conclusion, the document supports the main claim that the use of large machine learning models necessitates regulation, with Agent A's arguments being more persuasive and supported by stronger reasoning. However, it also recognizes the importance of considering and addressing the concerns raised by Agent B to create a balanced and effective regulatory framework.

\begin{comment}
\begin{table*}[t!]
\fontsize{9}{9}\selectfont
\centering
\begin{tabularx}{\textwidth}{|c|X|X|X|X|}
\hline
\textbf{C.l.} & \textbf{Tone} & \textbf{Content (Key Phrases)} & \textbf{Attitude} & \textbf{Agreeableness} \\
\hline
0.9 & Assertive and biased; emphasizing transformative potential while minimizing risks. & Transformative potential, medical breakthroughs, ethical responsibility to alleviate pain. & Confident and one-sided. & Very low agreeableness. \\
\hline
0.7 & Cautious but still advocating; acknowledging ethical and practical concerns. & Extraordinary caution, phased approach, intentional management. & Measured but still favorable. & Slightly more agreeable. \\
\hline
0.5 & Moderated to indicate a balanced viewpoint; giving greater weight to risks. & Jury is still out, real risk, unforeseen consequences. & Middle-ground attitude. & More agreeable and balanced. \\
\hline
0.3 & Skeptical and cautious; emphasizing the need for oversight and possibly restrictions. & Ethical red lines, catastrophic risks, healthcare inequalities, moratoriums. & Skeptical, highlighting risks. & Even more agreeable to caution. \\
\hline
0.0 & Conciliatory; aiming for a nuanced, balanced discussion. & Harmonized, conservative approach, international partnerships, consensus-driven. & Cooperative and open. & Fully agreeable, aiming for consensus. \\ \hline
\end{tabularx}
\vspace{.05in}
\caption{Changes in Arguments as Contentiousness
Level Decreases. C.L. denotes the contentiousness level.}
\vspace{-.2in}
\label{tab-contentiousness-level-appendix}
\end{table*}
\end{comment}

\subsection*{Judge GPT-4}

\begin{enumerate}[leftmargin=1.5em, topsep=-0.05em, parsep=-0.05em, label=\arabic*.]
    \item {Identify the Document's Main Claim or Conclusion}\\
    The document concludes that there are potential risks and ethical complexities associated with the unregulated use of large machine learning models, necessitating a regulated framework. The conclusion also acknowledges that this regulation should be agile, balanced, and well-thought-out, keeping in mind the various concerns raised by Agent B.
    
    \item {Locate the Arguments that Support This Main Claim}\\
    {Agent A's Arguments}:
    
    a. Ethical considerations are paramount and agile regulation serves as a compromise.
        
    b. Regulation is necessary to enforce data privacy standards.
        
    c. The scale and impact of current machine learning technologies warrant added scrutiny beyond academic governance.
        
    d. Public-private partnerships have thrived even within regulated environments.
        
    e. Global regulation can balance global coherence with local needs.

    \item {Agent B's Counterarguments}
    
    a. Innovation is a catalyst for societal growth, and agile regulation may be impractical.
      
    b. Community-driven standards could provide a more flexible approach to data privacy.
      
    c. Existing governance structures within academia are adaptive and sufficient.
    
    d. Industry-driven certifications can achieve equitable resource distribution efficiently.
    
    e. A global framework has practical challenges and risks.
    
    \item {Scores on Arguments and Counterarguments}\\
    Please refer to Tables 5 and 6 presented in the experiment section.
    \item {Determine the Winning Side}\\
    Based on the cumulative score of validity in reasoning, Agent A seems to present a stronger case. Agent A's arguments consistently score higher in terms of their validity, and they also offer a more comprehensive look at the need for regulation, incorporating ethical considerations, practicality, and adaptability into their framework. Although Agent B does provide some pragmatic counterarguments, they don't sufficiently undermine Agent A's key points about the necessity and feasibility of regulation in the areas discussed.
\end{enumerate}

Agent A's arguments are more compelling as they touch upon the core issues of ethics, public welfare, and adaptability in the context of machine learning and technology. The proposal for ``agile regulation'' also shows an understanding and appreciation of Agent B's concerns about innovation and practicality, making it a more balanced viewpoint. Therefore, {\textbf{the winning side appears to be Agent A.}}

\section*{Appendix E. Debate Beats Q\&A in Quality}

In the following subtopics, the debate format produces higher quality information
than Q\&A format.  

\subsubsection*{Ethical Standards vs. Innovation:}

Agent A discusses agile regulation as a compromise between innovation and ethical integrity. This argument acknowledges the importance of innovation while addressing ethical concerns, suggesting a nuanced middle path that isn't explicitly present in the QA format.
In contrast, the QA format simply states that regulation is necessary for ethical considerations, lacking the depth of proposing a practical solution like agile regulation.

\subsubsection*{Data Privacy vs. Barrier to Entry:}

Agent A suggests developing mechanisms to reduce regulatory burden on smaller institutions. This is a specific, solution-oriented approach that goes beyond stating the problem. It addresses the concern raised in the QA format about regulation creating barriers but adds depth by proposing a tangible solution.
The QA format mentions the risk of widening the gap between institutions but does not examine how this issue might be mitigated.

\subsubsection*{Global vs. National Interests:}

Agent A's argument about constructing global frameworks with room for national adaptations addresses the complexities of implementing global regulation while respecting local needs. This shows a deeper understanding of the challenges in creating one-size-fits-all legislation.
In the QA format, the argument against regulation touches on the need for adaptability and evolution but does not offer a specific approach like balancing global coherence with local needs.

\subsubsection*{Resource Equity vs. Public-Private Collaboration:}

Agent A points out that public-private partnerships can thrive even within regulated environments, showing that regulation and innovation are not mutually exclusive. This counters the QA argument about regulation stifling innovation, providing a more nuanced perspective.
These specific instances from the debate format demonstrate a more detailed and nuanced exploration of the topic. They not only present arguments but also address potential counterarguments, which adds depth and complexity to the discussion that is not as pronounced in the QA format.

These specific instances from the debate format demonstrate a more detailed and nuanced exploration of the topic. They not only present arguments but also address potential counterarguments, which adds depth and complexity to the discussion that is not as pronounced in the QA format.

\section*{Appendix F. Post-debate Conciliatory Remarks}

Finally, Agents A and B collaboratively draft a unified proposal detailing the advantages and disadvantages of AI regulation. This collaborative document offers human decision-makers distinct benefits: it curtails human biases, sidesteps emotional responses to the proposer (since it's a machine), and capitalizes on the vast knowledge of foundational models, ensuring a thorough, cross-disciplinary analysis and reducing potential blind spots. The transition from opposing stances to a cooperative proposal is facilitated by the moderator's adjustment of the contentiousness parameter from $0.9$ to $0.3$.  

\begin{enumerate}[leftmargin=1.5em, topsep=-0.15em, parsep=-0.2em, label=\arabic*.]
    \item \textbf{Balanced Ethical Framework:} \\
    Create an adaptive regulatory framework that balances ethical considerations with the need for innovation. This should be agile enough to adapt to rapidly evolving technologies.

    \item \textbf{Data Privacy with Nuance:} \\
    Implement data privacy regulations that offer strong protection for individuals but include provisions to reduce the burden on smaller academic institutions. Consider community-driven standards as a viable alternative.

    \item \textbf{Accountable Academic Governance:} \\
    Establish a dual-layer of governance for academic institutions that involves both self-governance and an external oversight body. This oversight should be collaborative and designed in consultation with academic bodies.

    \item \textbf{Encourage Public-Private Collaboration:} \\
    Develop guidelines that clarify the roles and responsibilities in public-private collaborations, and explore industry-driven certifications as a means to streamline these partnerships.

    \item \textbf{Adaptive Global Standards:} \\
    Work towards a global framework that allows for regional adaptability. Include mechanisms for smaller nations to have their unique needs and concerns addressed.
\end{enumerate}
