# Supplementary material for: Unlocking the Wisdom of Large Language Models: An Introduction to The Path to Artificial General Intelligence
Source: arXiv:2409.01007 source file (2025-04-15)
Supplement: Supplementary file 10 [file AppendixA-Metrics.tex]

\section*{Appendix A: Quality Metrics and Formulas}

\begin{table*}[th!]
\begin{small}
%\begin{customsize}
\centering
\begin{tabular}{|p{2.2cm}|p{3.8cm}|p{3.5cm}|p{4.8cm}|}
\toprule
\hline
\textbf{Metric} & \textbf{Pros} & \textbf{Cons} & \textbf{Remedies} \\
\hline
Cross Entropy (CE) \cite{Shore1980AxiomaticDO} & Measures how well the predictions of one model fit the actual distribution of another model’s outputs (asymmetric). & Computationally intensive especially with large models and data sets; sensitive to the exact nature of probability distributions. & Optimize computation strategies; use approximations or sampling methods to manage large data sets or complex models. \\
\hline 
Entropy Shannon \newline \cite{shannon1948} & Indicates level of diversity or predictability; high values suggest exploration of possibilities, and low for confidence on few choices & High entropy might indicate noise rather than useful diversity; low entropy might mask important variability. & Use critical reading methods (Appendix A) to assess argument quality; implement noise detection to differentiate between useful diversity and noise. \\
\hline
Jensen-Shannon \newline Divergence (JS) \newline \cite{lin1991divergence} & Symmetric and bounded (0 to 1), providing an interpretable measure of distributional differences. & May be less sensitive to small differences between distributions. & Increase sensitivity settings or resolution of the metric; combine with other metrics to capture finer distinctions between distributions. \\
\hline
KL Divergence \newline \cite{kullback1951information} & Measures diff. between two distributions; useful for comparing a model's dist. to a reference dist. & Asymmetric; not well-defined if the reference distribution has zero probabilities & Use smoothing techniques to avoid zero probabilities; consider symmetric alternatives like JS divergence \\
\hline
Mutual Info. \cite{Shore1980AxiomaticDO} & Measures reduction of uncertainty; symmetric. & Does not indicate the directionality of information flow. & Supplement with directional information metrics; normalized with max entropy of A and B. \\
\hline
Wasserstein \newline Distance (WD) \newline \cite{kantorovich1942translocation} & Direct measure of how similar or different the model outputs are; it depicts symmetric relationship.  & Not bounded but can be normalized or bounded for consistent interpretation. & Define context-specific bounds for low, medium, and high divergence; consider normalizing it for non-directional comparisons. \\
\hline
\bottomrule
\end{tabular}
\end{small}
%\end{customsize}
%\vspace{-0.1in}
\caption{Summary of metrics for assessing LLM debates (equations are presented in Appendix E)}
\label{tab:metrics}
%\vspace{-0.2in}
\end{table*}

Table \ref{tab:metrics} lists the metrics employed by EVINCE to quantify agreement, diversity, and mutual information, promoting productive information exchange and enhancing prediction quality. 
Measures such as Shannon entropy, Wasserstein distance (WD), Jensen-Shannon (JS) divergence, mutual information (MI), and cross-entropy (CE) are used complementarily. WD and CE are particularly valued for their ability to handle simplicity and information asymmetry, respectively.

The rest of this appendix outlines the mathematical formulas for various data analysis metrics used in probabilistic and statistical modeling. 

\subsection*{Kullback-Leibler Divergence}
The Kullback-Leibler Divergence measures the difference between two probability distributions:
\begin{small}
\[
D_{KL}(P \| Q) = \sum_{x \in \mathcal{X}} P(x) \log\left(\frac{P(x)}{Q(x)}\right).
\]
\end{small}
\subsection*{Jensen-Shannon Divergence}
The Jensen-Shannon Divergence is a symmetrized and smoothed version of the KL Divergence:
\begin{small}
\[
JSD(P \| Q) = \frac{1}{2} D_{KL}(P \| M) + \frac{1}{2} D_{KL}(Q \| M)
\]
where \( M = \frac{1}{2}(P + Q) \).
\end{small}
\subsection*{Wasserstein Distance}
The Wasserstein Distance, also known as the Earth Mover's Distance (EMD), measures the distance between two probability distributions:
\begin{small}
\[
W(P, Q) = \inf_{\gamma \in \Gamma(P, Q)} \int_{\mathcal{X} \times \mathcal{Y}} d(x, y) \, d\gamma(x, y).
\]
\end{small}
\subsection*{Cross Entropy}
Cross Entropy measures the average number of bits required to identify an event from a set of possibilities, under a specific model:
\begin{small}
\[
H(P, Q) = -\sum_{x \in \mathcal{X}} P(x) \log(Q(x)).
\]
\end{small}
\subsection*{Mutual Information}
Mutual Information measures the amount of information that one random variable contains about another random variable:
\begin{small}
\[
I(X; Y) = \sum_{y \in \mathcal{Y}} \sum_{x \in \mathcal{X}} p(x, y) \log\left(\frac{p(x, y)}{p(x)p(y)}\right).
\]
\end{small}
\subsection*{Normalized Mutual Information}
Normalized Mutual Information is calculated as the mutual information divided by the maximum of the entropies of the variables:
\begin{small}
\[
NMI(X; Y) = \frac{I(X; Y)}{\max(H(X), H(Y))}.
\]
\end{small}
\vspace{-.2in}
