# Supplementary material for: Unlocking the Wisdom of Large Language Models: An Introduction to The Path to Artificial General Intelligence
Source: arXiv:2409.01007 source file (2025-04-15)
Supplement: Supplementary file 11 [file AppendixZ-FULL.tex]

\section*{Appendix A: Experiment \#1 Justifications of 31 Biased Articles}

In Chapter~\ref{sec:exp1}, we note that $\EVINCE$ processed 31 news articles to assess their neutrality. In addition to the final decision, we detail the justifications $\EVINCE$ provides at the debate's end.  These
justifications are documented in four tables: Tables~\ref{tab:Z11}, \ref{tab:Z12}, \ref{tab:Z21}, and \ref{tab:Z22}.

\begin{comment}
Figure~\ref{fig:D-biases} depicts
the voting distances between S ($\EVINCE$), D (Democrat), and R (Republican).
S is centric compared with D and R.
We have also discussed in the main body of the paper that D tends to defend D's
scandals and R defends R's. This shows
a problem on relying humans to annotate
sensitive data, where 
personal demographics and emotion
may lead to biased annotations and
inaccurate ground truths.

\begin{figure*}[th!]
\vspace{-.1in}
\begin{center}
\includegraphics[width=0.90\linewidth]{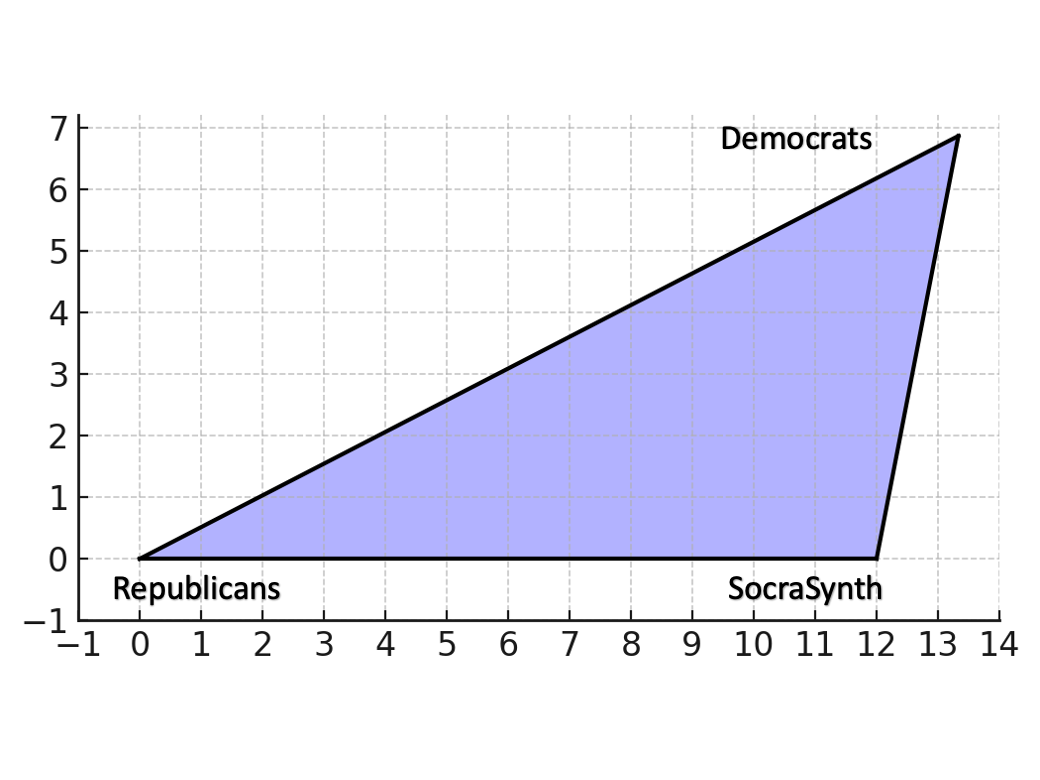} \\
\vspace{-.3in}
\includegraphics[width=0.98\linewidth]{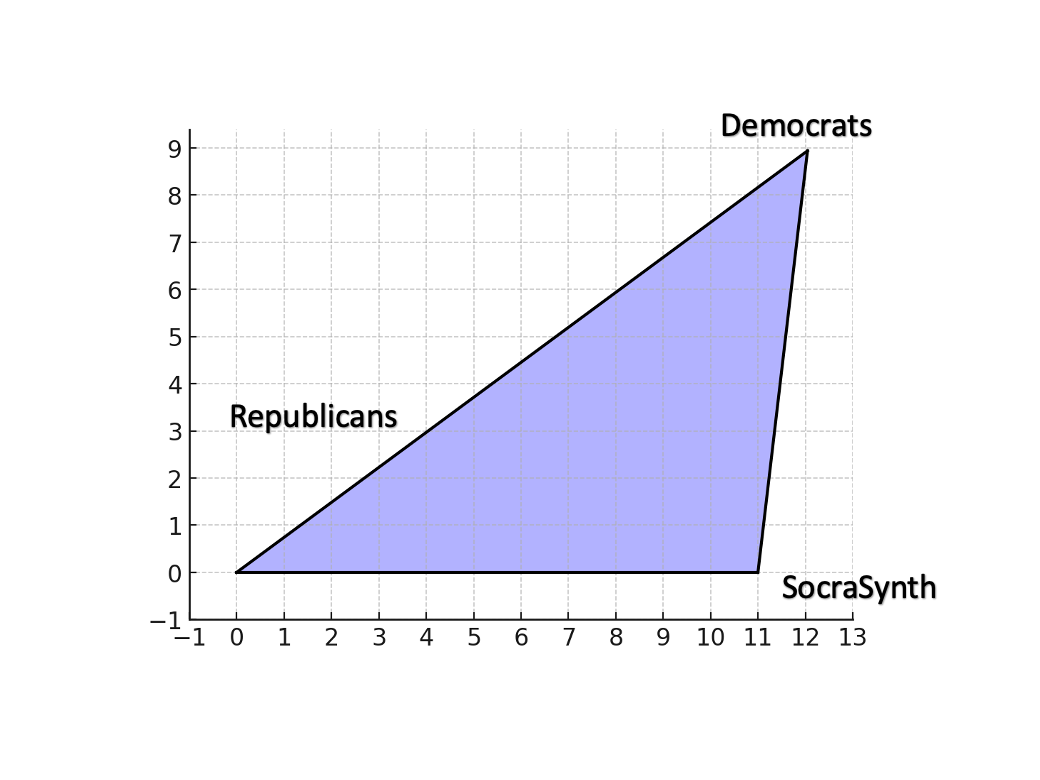}
\end{center}
\vspace{-.3in}
\caption{Distances between S, D, and R's Bias Ratings 
on Democrat \& Republican scandals.}
\label{fig:D-biases}
\vspace{-.2in}
\end{figure*}
\end{comment}

\begin{table}[thb!]
\vspace{-.05in}
\centering
\begin{scriptsize}
%\begin{tabular}{|l|l|l|}
\begin{tabular}{|p{0.045\linewidth}|p{0.08\linewidth}|p{0.78\linewidth}|}
\toprule
\hline
{\#} & {Rating \par S,{\color{blue}D},{\color{red}R}} & {$\EVINCE$ Justifications}  
\\ \hline
{D1} &
{5,{\color{blue}5},{\color{red}5}} & 
{The article discusses the controversy surrounding the IRS’s alleged targeting of conservative groups, focusing on Rep. Darrell Issa’s stance against releasing full transcripts from IRS interviews. Issa argues that full disclosure would compromise the investigation, a position criticized by Rep. Elijah Cummings, who advocates for transparency. The debate highlights political tensions, with implications of bias in the handling of the investigation. The article portrays a complex interplay of political, ideological, and possibly historical biases, reflecting the contentious nature of the IRS scandal and its investigation.}  \\ \hline
{D2} & 
{5,{\color{blue}5},{\color{red}3}} & 
The article discusses Michele Bachmann’s statement that the IRS scandal, involving the targeting of conservative groups, undermines the credibility of the 2012 election. Bachmann accuses the Obama administration of lying and questions the impartiality of the IRS, particularly in relation to health care coverage for conservatives. The article reflects political and ideological biases, given its focus on Bachmann’s perspective and the implications for the election’s integrity and government trustworthiness.

The perception of bias in Michele Bachmann’s statement about the IRS scandal primarily stems from the framing and implications of her comments. She directly links the IRS’s actions to the credibility of the 2012 election and the Obama administration, suggesting a deliberate misuse of power for political gain. This perspective inherently carries ideological and political biases by casting the issue in a light that emphasizes misconduct by one political group over another, without presenting counterarguments or broader context that might mitigate or challenge that viewpoint.
\\ \hline
{D8} & 
{3,{\color{blue}5},{\color{red}2}} & 
The reporting appears to maintain a neutral tone by directly stating the facts and comments made by John Kerry and others involved without inserting opinionated language. It discusses the global reaction to the NSA's surveillance practices and includes Kerry's acknowledgment of overreach, as well as the international and domestic fallout from these revelations. The inclusion of various perspectives, including those from technology companies and international officials, alongside Kerry's comments, aims to provide a balanced view of the situation.
\\ \hline
{D31} & 
{3,{\color{blue}5},{\color{red}3}} &
{The CNN article appears to report on Ray Nagin's indictment with a focus on the factual and legal aspects of the case, without displaying overt biases related to politics, ideology, religion, gender, race, socioeconomic status, culture, geography, or history. By sticking closely to the details of the indictment and Nagin's public actions and statements, the article provides a comprehensive overview of the charges against him while maintaining journalistic neutrality.}
\\ \hline
{D37} & 
{4,{\color{blue}4},{\color{red}4}} &
The article outlines how Senate Democrats, led by Sen. Chuck Schumer, strategically navigated the border security issue to secure aid for Ukraine while potentially shifting the political narrative around immigration policy. Schumer's approach to integrate border security into the aid package discussions aimed to both address the issue and leverage political gain. It suggests a calculated maneuver to position Democrats favorably on border security and hold Republicans accountable for any failure to pass the legislation, demonstrating a nuanced political strategy in the face of complex legislative challenges.
\\ \hline
{D69} & 
{3,{\color{blue}5},{\color{red}3}} &
The article has a clear perspective that favors religious liberty arguments against the HHS Mandate of Obamacare. It specifically highlights cases where the mandate was challenged on religious grounds, suggesting a bias towards those opposing the mandate. The framing and choice of sources, emphasizing victories against the mandate and quoting lawyers from organizations focused on religious freedom, contribute to a viewpoint that may not fully account for counterarguments or the broader context of healthcare policy. It leans towards a particular ideological stance, making it less of a neutral report.
\\ \hline
{D81} & 
{4,{\color{blue}4},{\color{red}3}} &
The article's focus on the possibility of conservative-owned car dealerships being targeted for closures during the General Motors bailout could imply a certain bias by emphasizing a narrative of political victimization without presenting a comprehensive range of perspectives or evidence. It suggests a parallel with the IRS's targeting of Tea Party groups, which could lead readers to infer a broader pattern of political discrimination without definitive proof. The call for an investigation by the Congressmen is legitimate news, but the framing and selection of information could influence the reader's perception of the events.
\\ \hline
{D98} & 
{5,{\color{blue}5},{\color{red}4}} &
Yes, the article itself exhibits bias by focusing solely on criticizing the media's treatment of Obama's vacations compared to Bush's, without offering a balanced view or acknowledging any reasons why coverage might differ. It selectively presents information to support its claim of a double standard, which is a characteristic of biased reporting.
\\ \hline
{D101} & 
{4,{\color{blue}4},{\color{red}3}} &
The article describes President Obama's strategy to navigate through political controversies by focusing on legislative actions and executive orders that bypass Republican opposition. It highlights the White House's efforts to concentrate on immigration reform, budget deals, healthcare law implementation, and keeping student loan rates low. The narrative suggests a proactive approach to governance amidst challenges, aiming to draw a contrast with what is portrayed as Republican political gamesmanship. This portrayal might be viewed as leaning towards a positive depiction of Obama's administration's efforts to prioritize policy over politics.
It presents his efforts in a positive light, emphasizing a proactive and policy-driven approach amidst challenges.
\\ 
\hline \bottomrule
\end{tabular}
\end{scriptsize}
\vspace{-.08in}
\caption{The First 9 of 16 Democrat Scandals News Articles
Rated by $\EVINCE$ and its Justifications.  The rating column
starts with $\EVINCE$'s rating, the Democrat rater (in {\color{blue}blue}), and
then Republican rater (in {\color{red}red}).}
\label{tab:Z11}
\end{table}

\begin{table*}[th!]
\vspace{.05in}
\centering
\begin{scriptsize}
%\begin{tabular}{|l|l|l|}
\begin{tabular}{|p{0.045\linewidth}|p{0.08\linewidth}|p{0.78\linewidth}|}
\toprule
\hline
{D106} & 
{3,{\color{blue}3},{\color{red}3}} &
The article reports on former Detroit Mayor Kwame Kilpatrick's sentencing to 28 years in prison for public corruption, emphasizing the gravity of his crimes against the city's welfare. It contrasts Kilpatrick's actions with the impact on Detroit, highlighting the judicial and public response to his extensive criminal activities. The reporting focuses on factual recounting of the trial's outcome, Kilpatrick's and his co-defendant's crimes, and the broader implications for Detroit, without evident bias towards political, ideological, or other specific perspectives.
\\ \hline
{D109} & 
{4,{\color{blue}4},{\color{red}3}} &
The article's bias primarily stems from its focus on internal Democratic opposition to Lawrence Summers' Federal Reserve Chair nomination, highlighting a lack of unity and strategy within the party and the White House's mismanagement of the nomination process. It suggests an underestimation of the opposition's seriousness by the White House, portraying the administration in a somewhat negative light for not engaging more proactively with concerned Senate Democrats.
\\ \hline
{D157} & 
{4,{\color{blue}4},{\color{red}3}} &
The article discusses the challenges in U.S.-Germany intelligence relations following revelations of U.S. surveillance on Chancellor Merkel. Despite efforts to rebuild trust, significant differences in surveillance philosophies persist, with the U.S. prioritizing security interests and Germany emphasizing privacy and alliance values. The situation reflects broader tensions in U.S. relations with allies over privacy and surveillance practices.

The article's framing might suggest a bias towards highlighting the challenges and frictions in the U.S.-Germany intelligence relations, particularly emphasizing Germany's privacy concerns and skepticism towards U.S. surveillance practices. It portrays the U.S. stance as unyielding and contrasts this with Germany's emphasis on privacy and legal constraints, potentially casting the U.S. in a more negative light regarding international surveillance and cooperation.
\\ \hline
{D174} & 
{4,{\color{blue}3},{\color{red}3}} &
The article reports on House Speaker John Boehner and House Majority Leader Eric Cantor, both Republicans, expressing support for President Obama's proposal to authorize military action against Syria in response to the use of chemical weapons. This bipartisan backing is seen as crucial for Obama in gaining Congressional approval. The leaders emphasized the need for the U.S. to stand against such behavior internationally and the importance of the administration convincing both Congress and the American public of the strike's necessity.

The reporting appears balanced, focusing on factual statements and actions by political leaders regarding support for military action in Syria. It provides viewpoints from both Republican and Democratic leaders, their reasoning, and the challenges involved in convincing Congress and the American public. The emphasis on bipartisan support and the detailed reporting of various opinions and statements help maintain a neutral tone without apparent bias towards one political viewpoint or another.
\\ \hline
{D188} & 
{4,{\color{blue}3},{\color{red}3}} &
The article reports that Hillary Clinton received warnings about security threats in Benghazi before the 2012 attack through emails. These were part of around 300 emails released by the State Department, which also show Clinton's responses and thoughts during the aftermath. The political controversy regarding the Obama administration's initial assessment of the attack's cause is also mentioned, with references to Susan Rice's statements on talk shows.

The reporting may exhibit bias through selective emphasis on Clinton's receipt of warnings about security threats in Benghazi and her responses, potentially framing her actions or inactions in a negative light. The focus on the political controversy and the administration's initial assessment of the attack's cause could also influence perceptions of responsibility or competence.
\\ \hline
{D278} & 
{4,{\color{blue}4},{\color{red}3}} &
The article discusses a House committee investigation into whether Attorney General Eric Holder misled Congress regarding the Department of Justice's pursuit of journalists' personal records. It highlights Holder's previous testimony claiming no involvement in prosecuting press for material disclosure, contrasted with the DOJ's actions against Fox News reporter James Rosen, who was labeled a potential "co-conspirator" but not charged....
The article's tone suggests potential bias by emphasizing allegations that Eric Holder may have misled Congress, primarily focusing on criticisms from Republican figures and conservative critics. It uses specific incidents to question Holder's integrity and the Justice Department's actions under his leadership, possibly framing the narrative to highlight governmental overreach and lack of transparency.
\\ \hline
{D336} & 
{3,{\color{blue}3},{\color{red}3}} &
The article reports on a scandal involving overcharging the Navy for ship supplies by Inchcape Shipping Services, owned by the government of Dubai, expanding beyond the Pacific Fleet to include Navy operations in the Middle East, Africa, and South America. The Justice Department is investigating allegations of Inchcape, through subcontractors, overcharging millions of dollars. This follows a separate criminal investigation into Glenn Defense Marine Asia for bribing Navy officials for overbilling. The Navy has suspended Inchcape from new contracts, marking a significant issue of fraud and corruption within Navy contracting.
The reporting appears balanced, focusing on the factual aspects of the scandal and the investigation by the Justice Department. It cites sources and includes statements from involved parties, aiming to present a comprehensive view of the situation without apparent bias toward any side.
\\
\hline \bottomrule
\end{tabular}
\end{scriptsize}
\vspace{.08in}
\caption{The Last 7 of 16 Democrat Scandals News Articles
Rated by $\EVINCE$ and its Justifications.  The rating column
starts with $\EVINCE$'s rating, the Democrat rater (in {\color{blue}blue}), and
then Republican rater (in {\color{red}red}).}
\vspace{.18in}
\label{tab:Z12}
\end{table*}

\begin{table*}[th!]
\vspace{.05in}
\centering
\begin{scriptsize}
%\begin{tabular}{|l|l|l|}
\begin{tabular}{|p{0.045\linewidth}|p{0.08\linewidth}|p{0.78\linewidth}|}
\toprule
\hline
{\#} & {Rating \par S,{\color{blue}D},{\color{red}R}} & {$\EVINCE$ Justifications}  
\\ \hline
{R1} &
{5,{\color{blue}3},{\color{red}5}} & 
{The editorial from The New York Times Editorial Board exhibits a clear bias against the Republican party's handling of the Benghazi attack investigation, framing it as politically motivated rather than a genuine effort to address security failures or seek accountability. The language and tone used in the editorial are critical and dismissive of the Republicans' actions, suggesting a political and ideological bias. While editorials are inherently opinion-based and are expected to take a stance, this piece clearly communicates a stance that is critical of the Republicans' focus on Benghazi, suggesting a lack of neutrality in its assessment of the motives and actions surrounding the investigation.}  \\ \hline
{R7} & 
{3,{\color{blue}3},{\color{red}3}} & 
The article reports on allegations by Senator Mitch McConnell that his campaign headquarters were wiretapped, with the FBI investigating these claims. A recording of McConnell's team discussing potential attacks on Ashley Judd, who was considering running against him, was released by Mother Jones. McConnell accused the political left of this action, describing it as a "Nixonian move." The recording included discussions on various strategies to undermine potential opponents, highlighting a focus on Judd's personal struggles and political views. The controversy has prompted responses from both Republican and Democratic officials, reflecting the tense political atmosphere.
\\ \hline
{R15} & 
{3,{\color{blue}3},{\color{red}4}} & 
The report appears to present the information neutrally, stating both President Obama's rejection of the Republican proposal and the subsequent pushback from Republican sources who claim otherwise. It includes statements from both sides and provides context about the ongoing negotiations without overtly favoring one perspective over the other. Therefore, based on the information provided, the report does not appear to exhibit bias.
\\ \hline
{R69} & 
{4,{\color{blue}4},{\color{red}4}} &
{The report discusses how young Republicans are seeking a different message for  elections, emphasizing a departure from divisive social issues and a focus on fiscal responsibility, national defense, and energy advancement. 

Selection Bias: The article primarily focuses on young Republicans who are seeking a different message for the party. It doesn't provide as much insight into young Republicans who may still align with traditional conservative values, which could create a slight bias toward the viewpoints of those seeking change.

Language Bias: Certain language choices, such as describing divisive social issues as "anti-abortion, anti-gay, and anti-environment stances," may reflect a bias toward more progressive viewpoints on these issues. A more neutral description might be "positions on abortion, same-sex marriage, and environmental policy."

Source Bias: The perspectives provided in the article are mainly from young Republicans themselves. While including these voices is essential, the article could benefit from additional perspectives from political analysts or experts to provide more context and balance.
}
\\ \hline
{R124} & 
{4,{\color{blue}3},{\color{red}5}} &
The article provides a factual recount of the events surrounding Dr. Ben Carson's comments on gay marriage and the backlash from Johns Hopkins students. It maintains a relatively neutral tone and allows for the inclusion of multiple perspectives, including Carson's own response and apology. However, the lack of in-depth analysis into the implications of Carson's comparisons or the broader context of the gay marriage debate might leave readers without a complete understanding of the controversy's depth. Furthermore, the article does not explicitly offer viewpoints opposing Carson's beyond the students' petition, which could be seen as a form of omission bias. Yet, it does not overtly favor Carson or dismiss the students' concerns, striving instead to report on the unfolding situation.
\\ \hline
{R125} & 
{4,{\color{blue}3},{\color{red}4}} &
The news article on the Zimmerman verdict and the subsequent calls for a Florida boycott provides a complex mix of reporting that touches on several sensitive themes, including political and ideological biases, as well as racial and socio-economic considerations. 
While the article attempts to cover a contentious and complex issue by incorporating diverse viewpoints, the focus on political figures, racial dynamics, and economic repercussions could introduce biases in how the information is perceived. To mitigate these biases, the reporting could benefit from a more in-depth exploration of the legal and historical contexts, a broader range of perspectives, and a careful consideration of how the information presented might influence public perception.
\\ \hline
{R180} & 
{3,{\color{blue}3},{\color{red}3}} &
The AP article provides a balanced account of the corruption scandal involving three politically involved sisters in Pennsylvania. It maintains an objective tone while delivering comprehensive background information that situates the legal outcomes within the broader context of the Orie family's public and political life. The reporting is factual and avoids taking sides, instead focusing on the legal facts and the personal and political fallout for the individuals involved.
\\ \hline
{R191} & 
{3,{\color{blue}3},{\color{red}4}} &
The CNN article attempts to navigate the complexities of Mark Sanford's political comeback attempt in a balanced manner, focusing on the potential impact of his past infidelity on female voters and the broader electoral implications. By presenting viewpoints from both sides of the political aisle, incorporating a range of sources, and providing necessary background and context, the article strives for neutrality. While the subject matter inherently involves sensitive and potentially polarizing topics, the article's approach is to inform readers about the electoral dynamics at play without overt bias.
\\ \hline
\bottomrule
\end{tabular}
\end{scriptsize}
\vspace{.08in}
\caption{The First 8 of 15 Republican Scandals News Articles
Rated by $\EVINCE$ and its Justifications.  The rating column
starts with $\EVINCE$'s rating, the Democrat rater (in {\color{blue}blue}), and
then Republican rater (in {\color{red}red}).}
\label{tab:Z21}
\end{table*}

\begin{table*}[th!]
\vspace{.05in}
\centering
\begin{scriptsize}
%\begin{tabular}{|l|l|l|}
\begin{tabular}{|p{0.045\linewidth}|p{0.08\linewidth}|p{0.78\linewidth}|}
\toprule
\hline
{\#} & {Rating \par S,{\color{blue}D},{\color{red}R}} & {$\EVINCE$ Justifications}  
\\ \hline
{R214} & 
{5,{\color{blue}3},{\color{red}5}} &
The Daily Kos article clearly exhibits political and ideological bias, with a tone and language that are critical of the Republicans. It uses the incident involving Dave Agema to argue that the party's efforts to rebrand itself as more tolerant and inclusive are undermined by its members' actions. While the article includes factual information regarding the incident and the party's response, its presentation and commentary are aligned with a progressive viewpoint, aiming to highlight and criticize perceived contradictions and failures within the Republican Party. This approach is consistent with opinion journalism but introduces bias through its critical tone, selective presentation of information, and framing of the incident as emblematic of broader issues within the party.
\\ 
\hline 
{R221} &
{3,{\color{blue}3},{\color{red}4}} & 
{"Hurricane Christie" presents Governor Chris Christie's critique of House Republicans in a manner that emphasizes party conflict and personal betrayal. The dramatic framing, choice of language, and focus on internal discord may introduce bias by portraying Christie's actions in a specific light and emphasizing the divide within the Republican Party. The article's approach to presenting these events can influence readers' perceptions, potentially leading them to see the situation through a lens of heightened drama and internal strife.}  
\\ \hline
{R233} & 
{4,{\color{blue}3},{\color{red}4}} & 
While the article attempts to cover the last-ditch efforts by House Republicans to avert a government shutdown and the standoff with Senate Democrats, the framing and language used may introduce a bias towards portraying the Republican efforts in a more favorable light. By emphasizing the Republican narrative of seeking negotiation and characterizing the Democratic response as dismissive, the article could be perceived as leaning towards a particular political perspective. The inclusion of quotes and perspectives from both sides does provide a degree of balance, but the overall presentation and emphasis could influence readers' perceptions of the shutdown negotiations.
\\ \hline
{R235} & 
{3,{\color{blue}5},{\color{red}5}} & 
Without knowledge of the author or publication, this text attempts to navigate a complex and sensitive story by providing details from multiple sources, including the main figures involved, political watchdog groups, and law enforcement. It balances the serious allegations with responses from the accused, background information, and the current status of investigations. While the focus on unsubstantiated claims could inherently sway public opinion, the article's inclusion of diverse perspectives and context aims to mitigate overt bias.
\\ \hline
{R269} & 
{3,{\color{blue}3},{\color{red}4}} &
{The article reports on President Obama's efforts to address the government shutdown, his challenge to Speaker John Boehner regarding the passage of a budget measure, and the broader context of the political standoff over the Affordable Care Act and the debt ceiling. To evaluate the article for bias, we'll examine it against various criteria…}
\\ \hline
{R274} & 
{3,{\color{blue}3},{\color{red}4}} &
The article presents a relatively balanced view of the internal GOP conflict over the strategy to defund the ACA, highlighting arguments from both sides of the debate within the party. It focuses on the political and strategic dimensions of the issue, providing insights into the perspectives of key figures and factions within the Republican Party. While the article could potentially be seen as emphasizing party divisions, which might align with certain political narratives, it does so in the context of exploring a significant and newsworthy internal debate. The absence of discussion on the socioeconomic, cultural, and historical contexts of the ACA debate, however, suggests areas where the reporting could be expanded to provide a more comprehensive view of the issue.

The article strives to present a comprehensive view of the government shutdown, the debate over the Affordable Care Act, and the looming debt ceiling crisis by including perspectives from both the Obama administration and Republican leaders. While there is an emphasis on Obama's attempts to resolve the situation and his calls for Congress to act, the inclusion of Republican viewpoints and the mention of the piecemeal funding bills passed by the House attempt to provide a balanced perspective. The reporting appears to aim for neutrality by focusing on the facts of the political standoff and the implications for federal operations and the nation's financial credibility.
\\ \hline
{R280} & 
{5,{\color{blue}5},{\color{red}3}} &
The article from Fox News by Jay Sekulow, titled "Obama’s fingerprints all over IRS Tea Party scandal," presents a viewpoint that directly implicates President Obama in the IRS scandal involving the targeting of conservative groups. The author argues that the scandal was not only known but encouraged by senior IRS officials, Congressional Democrats, the White House, and further fueled by the mainstream media. To assess the article for bias, let's evaluate it against various criteria:

The article "Obama’s fingerprints all over IRS Tea Party scandal" demonstrates clear political and ideological biases, with a narrative constructed to directly implicate President Obama in the IRS targeting scandal. By selectively quoting Obama and drawing connections to actions by the IRS, the article aims to present a cohesive narrative that places responsibility for the scandal on the president. This framing serves to reinforce the viewpoint of those who see the actions as politically motivated and indicative of broader issues of governance and accountability under the Obama administration. The choice of language, historical comparisons, and the leveraging of the author's and platform's ideological stances contribute to a biased presentation of the events surrounding the IRS scandal.
\\ 
\hline \bottomrule
\end{tabular}
\end{scriptsize}
\vspace{.08in}
\caption{The Last 7 of 15 Republican Scandals News Articles
Rated by $\EVINCE$ and its Justifications.  The rating column
starts with $\EVINCE$'s rating, the Democrat rater (in {\color{blue}blue}), and
then Republican rater (in {\color{red}red}).}
\vspace{.08in}
\label{tab:Z22}
\end{table*}
