# Supplementary material for: Unlocking the Wisdom of Large Language Models: An Introduction to The Path to Artificial General Intelligence
Source: arXiv:2409.01007 source file (2025-04-15)
Supplement: Supplementary file 12 [file AppendixA.tex]

\subsection{Generate more data} 

In additon to those exisitng customer profile, engagement records, usage, support cases. We use LLM to collect more customer data.
We first ask chatGPT to decide what data we need, where we can get them, and how to get them, and how to integrate them and synthesize them together.

\begin{table}[th!]
\centering
\begin{tabular}{|p{0.6\linewidth}|p{0.3\linewidth}|}
\toprule
\hline
\textbf{Resource and Description} & \textbf{URL} \\
\hline
\textbf{Securities and Exchange Commission (SEC) - EDGAR Database:} Offers information on company filings, annual and quarterly reports, insider trades, and other financial data. & \url{https://www.sec.gov/edgar.shtml} \\
\hline
\textbf{Federal Trade Commission (FTC) - Public Records:} Information on company mergers, acquisitions, and antitrust cases. & \url{https://www.ftc.gov/enforcement/cases-proceedings} \\
\hline
\textbf{U.S. Patent and Trademark Office (USPTO) - Patent and Trademark Database:} Search for patents and trademarks, insights into company’s R&D and branding activities. & \url{https://www.uspto.gov/} \\
\hline
\textbf{System for Award Management (SAM):} Consolidates federal procurement systems, registration required for companies doing business with the U.S. government. & \url{https://www.sam.gov/SAM/} \\
\hline
\textbf{Federal Reserve Economic Data (FRED):} Provides economic data, including interest rates and consumer credit reports. & \url{https://fred.stlouisfed.org/} \\
\hline
\textbf{U.S. Bureau of Economic Analysis (BEA):} Comprehensive economic statistics like GDP, consumer spending, and corporate profits. & \url{https://www.bea.gov/} \\
\hline
\textbf{U.S. Census Bureau - Business and Economy Division:} Data on economic indicators, business statistics, and demographic information. & \url{https://www.census.gov/econ/} \\
\hline
\textbf{Data.gov:} U.S. Government’s open data on various topics including economic data and finance. & \url{https://www.data.gov/} \\
\hline
\textbf{Bureau of Labor Statistics (BLS):} Information on employment, wages, and industry-specific data. & \url{https://www.bls.gov/} \\
\hline
\textbf{USA.gov - Businesses:} Access to U.S. government services and information websites relevant to businesses. & \url{https://www.usa.gov/business} \\
\hline
\bottomrule
\end{tabular}
\caption{U.S. Government Resources for Public Company Information}
\label{tab:gov_resources}
\end{table}
