# Supplementary material for: Unlocking the Wisdom of Large Language Models: An Introduction to The Path to Artificial General Intelligence
Source: arXiv:2409.01007 source file (2025-04-15)
Supplement: Supplementary file 13 [file AppendixX.tex]

%\newpage
\section{Appendix B: Additional Experiments}
\label{sec:more_experiments}

\begin{table}[ht!]
\centering
\begin{footnotesize}
\begin{tabular}{|l|p{0.8cm}|p{1.5cm}|p{1.1cm}|p{1.1cm}|p{1.1cm}|}
\toprule
\hline
\textbf{Play \#} & {Tactic \par Align.} & {Client \par Engagmnt} & {Action- \par able} & {Data \par Support} & {Reason \par Quality} \\ \hline
{\bf T0021}  & 7 & 6  & 6  & 7  & 7 \\
{\bf T0020/T0021} & 9 & 8 & 8 & 8 & 9 \\ \hline
\bottomrule
\end{tabular}
\end{footnotesize}
\caption{Before and After Play(s) for Customer Visit.}
\vspace{-.2in}
\label{tab:T0021vsT0020-0021}
\end{table}

The presentation of this experiment was divided into two parts as outlined by SocraPlan. Initially, we prompted Agent A to suggest a play for an upcoming onsite visit with customer Company\_51, which was identified as a key tactic in the sales playbook. After Agent A had submitted a proposal utilizing GPT-4, we proceeded with the second part of SocraPlan, orchestrating a debate between Agents A and B to further refine the play.

\subsection{Propose Play(s) for Tactic Customer Visit}

In our upcoming sales visit, we aim to provide Company\_51 with a comprehensive understanding of their product usage and cybersecurity defenses. Leveraging our Technique {\em T0021}: {\em Usage Analytics and Reporting}, we will present a detailed analysis of their engagement with our product, highlighting areas of improvement and aligning their defenses with the latest threat landscape. Our goal is to optimize their cybersecurity posture, ensuring they are well-equipped to handle emerging threats. We believe that this personalized approach, grounded in real data and insights, will not only enhance their product experience but also strengthen their overall cybersecurity resilience. Join us for this insightful session as we examine the specifics of your product usage and work together towards a more secure future.

\subsection*{Visit Agenda Proposal}

Reflecting on the available information, Agent A recommended
the following meeting agenda:

\begin{enumerate}[leftmargin=1.25em, topsep=.1em, parsep=.1em, label=\arabic*.]
\item \textit{0-10 mins: TA07: Optimization (T0021)} \\
Introduction and overview of the session's objectives, emphasizing the importance of product usage analytics in optimizing cybersecurity defenses.
\item \textit{10-30 mins: TA07: Optimization (T0021)} \\
Presentation of the comprehensive usage analytics report, highlighting Company\_51's product usage, engagement scores, and recent support cases (Ref 1 \& 4).
\item \textit{30-50 mins: TA07: Optimization (T0021)} \\
Discussion on the latest threat landscape (Ref 2), aligning Company\_51's current product usage with the protection against these threats, and identifying gaps in their defenses.
\item \textit{50-70 mins: TA07: Optimization (T0021)} \\
Demonstration of how to use the Vision One product to manage their attack surface, detect threats, and automate response options, addressing any concerns and providing solutions.
\item \textit{70-90 mins: TA07: Optimization (T0021)} \\
Summary of the discussion, next steps, and provision of additional resources or training materials as needed to help Company\_51 implement the recommendations.
\end{enumerate}

\subsection{Debate and Refine Proposed Play(s)}

After the debate between two GPT-4 agents, the second play (technique) 
{\em T0020} was added to {\em T0021} for the customer visit tactic.  The following is
the output generated by SocraSynth.

For our upcoming sales visit, we aim to give Company\_51 a clear understanding of their product usage, settings, and cybersecurity. Using Technique {\em T0021}: {\em Usage Analytics and Reporting}, we'll analyze their product interaction, identify areas for improvement, and align their security with current threats. Additionally, Technique {\em T0020}: {\em Using Playbooks} will help improve their response to Ransomware, enhancing their security strategy. Our goal is to strengthen their cybersecurity, preparing them to handle new threats. We look forward to working with Company\_51 in this session to enhance their product safety and security.

\subsection*{Visit Agenda Refinement}

\begin{enumerate}[leftmargin=1.25em, topsep=.1em, parsep=.1em, label=\arabic*.]
    \item \textit{0-10 mins: TA07: Optimization (T0021)} \\
    Kick-off with an introduction and session overview, underlining the critical role of product usage analytics and configuration in fortifying cybersecurity defenses.
    
    \item \textit{10-30 mins: TA07: Optimization (T0021)} \\
    Presentation on the detailed usage analytics report, showcasing Company\_51's product utilization, configuration, engagement metrics, and recent support incidents.
    
    \item \textit{30-50 mins: TA07: Optimization (T0021)} \\
    Engage in discussions concerning the current threat landscape, align Company\_51's product use and configurations with adequate protections, and pinpoint defense shortcomings.
    
    \item \textit{50-70 mins: TA07: Optimization (T0020)} \\
    Demonstrate the configuration and deployment of automated playbooks with the Vision One product, incorporating real-world scenarios pertinent to Company\_51's operations for a more relevant and captivating presentation.
    
    \item \textit{70-90 mins: TA07: Optimization (T0020)} \\
    Guide Company\_51 in crafting a simulated ransomware attack scenario and establishing an automated playbook for its resolution. Ensure comprehensive understanding and independent execution capability.
\end{enumerate}

%\subsection*{Remarks}

%This session is dedicated to delving into the specifics of Company\_51's product usage, with a collective aim of moving towards a fortified cybersecurity framework. Our goal is to ascertain that Company\_51 is well-prepared to confront and mitigate the risks presented by the evolving landscape of digital threats.

\subsection{Evaluation}

We assessed the original play {\em T0021} against the enhanced plays {\em T0021 \& T0020}, using the evaluation criteria outlined in Section~\ref{sec:casestudy9}.

\begin{enumerate}[leftmargin=1.25em, topsep=.1em, parsep=.1em, label=\arabic*.]
\item {\em Alignment with the tactic}: The degree to which the play corresponds with the intended tactic to achieve the strategic objective.
\item {\em Engagement with customer}: The play's effectiveness in engaging the customer.
\item {\em Actionability}: The feasibility and applicability of the play(s).
\item {\em Data support}: The level of factual data backing the play.
\item {\em Reasoning quality}: The strength of support reasoning. 
\end{enumerate}

Table~\ref{tab:T0021vsT0020-0021} presents the evaluation
results conducted by using CRIT.
The analysis revealed that the enhanced plays scored higher across all metrics, notably in actionability. This improvement is primarily due to play {\em T0020}, which incorporates training and drills into the session, offering customers practical experience in utilizing product features to counter cyber threats.
