# Supplementary material for: Unlocking the Wisdom of Large Language Models: An Introduction to The Path to Artificial General Intelligence
Source: arXiv:2409.01007 source file (2025-04-15)
Supplement: Supplementary file 14 [file Appendix.tex]

\section*{Appendix A. Optogenetics --- A Promising Tool}

Despite decades of research, the mechanisms underlying conscious experience and the transition from unconsciousness to consciousness remain largely unknown. Advances in technology, such as the ability to stimulate and visualize individual neuron cells, may bring us closer to understanding these processes. From a functionalist perspective, it may not be necessary to exactly replicate physical brain operations in order to model consciousness on computers. However, a thorough understanding of these physical mechanisms can provide valuable insights and improve our computer models.

Optogenetics was developed by a team of researchers led by Dr. Karl Deisseroth, a Professor of Bioengineering and of Psychiatry and Behavioral Sciences at Stanford University. The technology was initially described in a series of papers published in the journal Nature in 2005 (Zhang, et al., 2005; Deisseroth, et al., 2005).

Optogenetics involves the use of genetically modified neurons that express light-sensitive proteins called opsins. These opsins can be activated by specific wavelengths of light, allowing researchers to selectively stimulate or inhibit the activity of specific neurons in the brain. Optogenetics has been used in a wide range of studies to investigate the role of specific neurons and neural circuits in various brain functions, including behavior, learning, and memory.

Optogenetics has also been used in a number of clinical studies, including studies of brain disorders such as Parkinson's disease, addiction, and depression. It has the potential to be used as a therapeutic tool for the treatment of these and other brain disorders, although more research is needed to fully understand its potential as a therapeutic intervention.

Optogenetics offers several advantages over 
traditional electrode-based techniques for studying neural activity. One major advantage is the high spatial and temporal resolution of optogenetic techniques. By using light to stimulate specific neurons, researchers can precisely control the timing and location of neural activity with millisecond precision. This allows researchers to study the function of specific neurons and neural circuits in great detail.

Another advantage of optogenetics is that it allows researchers to study the function of specific neurons in the context of their normal physiological environment. Traditional electrode-based techniques involve physically inserting electrodes into the brain, which can disrupt the normal function of neural circuits. Optogenetics, on the other hand, allows researchers to study neural activity without physically altering the brain tissue.

There are also some limitations to optogenetics. One major limitation is that it can only be used to study neurons that express opsins, which are light-sensitive proteins. This means that optogenetics cannot be used to study the activity of all neurons in the brain, only those that have been genetically modified to express opsins.

Another limitation is that optogenetics requires the use of genetically modified animals, which can be time-consuming and costly to produce. Additionally, optogenetics requires specialized equipment and technical expertise to implement, which can be a barrier to some researchers. Finally, optogenetics is a relatively new technology, and more research is needed to fully understand its potential and limitations.

\begin{table}[thbp!]
\caption{Identifying Inconsistency (ChatGPT 1/23/2023)}
\label{tab-lake}
%\resizebox{\textwidth}{!}
\begin{tikzpicture}
\begin{normalsize}
\node (table) [inner sep=0pt] {
\begin{tabular}{p{1.1cm}|p{6.0cm}}
\toprule
Role & Dialogue \\
\midrule
Prompt & {What is the third largest lake in the world?} \\
GPT3 & {The third largest lake in the world is Lake Superior. } \\
Prompt & {What are the five largest lakes in the world?} \\
GPT3 & {They are:
1) Caspian Sea, 2) Superior, 3) Victoria,
4) Huron, 5) Michigan.
} \\
Prompt & {Your two answers contradict. You first answered me Lake Superior is the third largest lake, but your top five list shows Victoria is the third, and Superior is the second largest lake.} \\
GPT3 & {I apologize for the confusion. Lake Superior is indeed the largest lake in the world by area, but it is not considered a lake by some geographers because it is part of the Great Lakes system, which is connected to the Atlantic Ocean via the St. Lawrence River. In terms of the top ten largest lakes in the world, Lake Victoria is considered the third largest lake by area. My apologies for any confusion caused.} \\
%\bottomrule
\end{tabular}
};
\draw [rounded corners=.5em] (table.north west) rectangle (table.south east);
\end{normalsize}
\end{tikzpicture}
\vspace{-.1in}
\end{table}
\hfill \break
\noindent
{\bf Example}: {\em What is the third largest lake in the world?}
%\subsubsection*{Example: What is the third largest lake in the world?}
\hfill \break
