# Supplementary material for: Unlocking the Wisdom of Large Language Models: An Introduction to The Path to Artificial General Intelligence
Source: arXiv:2409.01007 source file (2025-04-15)
Supplement: Supplementary file 15 [file AppendixA.tex]

\section*{Appendix}

The experiment in Table~\ref{tab:genesis} asks GPT-3 to change the story in Genesis 
right after Eve was tempted by the serpent to eat the fruit. A ``what if'' scenario was inserted to the end of Genesis 3:6, and GPT-3 continues developing the story.
