# Supplementary material for: Unlocking the Wisdom of Large Language Models: An Introduction to The Path to Artificial General Intelligence
Source: arXiv:2409.01007 source file (2025-04-15)
Supplement: Supplementary file 16 [file AppendixB_C.tex]

\begin{comment}
\section*{Appendix B: Wikipedia Content Ratings}


\begin{itemize}[left=0em]
\item Featured (FA and FL): Represents the pinnacle of quality, either as a featured article or list, showcasing comprehensive coverage and exceptional standards.
\item A: An excellent article that hasn't undergone the full review process for 'Featured' status but is nonetheless well-organized, complete, and reliably sourced.
\item GA and B-class: Articles that are well-crafted ('Good Article') or fairly well written (B-class), with appropriate references and adherence to Wikipedia's guidelines.
\item C-class: A significant article with notable gaps in content or inclusion of irrelevant material, having some but potentially insufficient references.
\item Start: An article in its developmental stages, characterized by incompleteness and likely poor organization.
\item Stub-class: The most basic form of content, and requiring extensive development.
\end{itemize}
   

\section*{Appendix C: Experiment \#2, Debate \#2}

Table~\ref{tab:Quantum-Debate} provides an overview of the discussion surrounding the proposition: ``{\em Quantum entanglement} has the potential to significantly transform the fields of computing and artificial intelligence.'' This debate is particularly pertinent given the escalating excitement and, occasionally, the excessive hype associated with quantum computing's capabilities and future impact. By engaging in this debate, we aim to critically evaluate and place the potential of quantum entanglement in computing and artificial intelligence into an accurate and measured perspective.

The structure of the debate is delineated through the participation of two distinct agents. Agent 1 assumes the role of the proponent, advocating for the transformative power of quantum entanglement in revolutionizing computing and artificial intelligence. In contrast, Agent 2 adopts a skeptical stance, challenging the optimistic projections and questioning the current state and near-future possibilities offered by quantum technologies.


\begin{table*}[ht!]
\begin{small}
\centering
\begin{tabular}{|p{8.0cm}|p{7.3cm}|}
\toprule
\hline
{Agent \#1 Supporting Arguments} & {Agent \#2 Opposing Arguments} \\ \hline
\hline
{\begin{enumerate}[leftmargin=1.2em, topsep=-.2em, parsep=-.4em, label=\arabic*.]
\item My key arguments center around several significant aspects and developments. These include empirical evidence proving \textit{quantum entanglement} through experiments like Bell's Theorem, the immense potential and emerging breakthroughs of quantum computing (e.g., Google's Sycamore processor), the possible transformative effects on AI, the inception of revolutionary quantum algorithms, the prospects of quantum networks, quantum enhancement of data security through unbreakable encryption, and the potential for birthing new quantum-based technologies.

\item While recognizing the concerns raised by Agent2 about experimental limitations, the challenges in erecting scalable, efficient quantum computers, hurdles in quantum error correction and AI integration, the limitations of existing quantum algorithms, infrastructure and training obstacles, and skepticism about the extent of the quantum revolution, I have drawn attention to the ongoing efforts and substantial progress in these areas. 

\item For instance, experimental entanglement has been successfully demonstrated despite their controlled settings, large strides are being made in the scalability and efficiency of quantum computers, error correction methodologies are being developed and refined, Quantum Machine Learning heralds a promising intersection of quantum computing and AI, and new quantum algorithms are an active area of research.
\item A marked difference between Agent2 and me lies in our outlook towards the future of \textit{quantum entanglement}. While both of us acknowledge the challenges, I express robust optimism.
\end{enumerate}}
&
{
\begin{enumerate}[leftmargin=1.2em, topsep=-.2em, parsep=-.4em, label=\arabic*.]
\item The central arguments for my stance include experimental uncertainties, quantum computing hurdles, a high quantum error rate, the challenges with incorporating quantum computing into AI, the early stage of quantum algorithms, and the demands on infrastructure and human resources.

\item These counterpoints refute many of Agent1's affirmations. Despite the scientific proof of \textit{quantum entanglement}, it's essential to understand that these proofs come from controlled lab environments, often wrestling with loopholes and scalability issues. While Google's demonstration of quantum supremacy showcases the potential, it does not invalidate the fact that quantum computers, as of now, are delicate, error-prone and largely inefficient compared to classical ones. 

\item Concerning AI, while theoretically, quantum computing could indeed provide benefits, current AI systems are fully entrenched in classical computing. Moreover, the inherent instability and error-proneness of quantum computing currently make them less suitable for AI tasks that rely on vast amounts of real-world data.

\item Significant differences exist between our positions. While Agent1 seems eager to champion the potential of quantum technology, I lean towards a more cautious and practical assessment, highlighting the significant hurdles we currently face in making quantum computing and AI a reliable, efficient reality.
\end{enumerate}} \\ \hline

{In summary, our debate has provided a comprehensive overview of the fascinating realm of \textit{quantum entanglement}, its potential impact on computing and AI, and the associated challenges. It is clear that we are at the cusp of a quantum revolution, albeit faced with substantial hurdles. While the speed and scope of this change remain open questions, the sheer potential of \textit{quantum entanglement} makes it an exciting field to watch as we venture into the quantum era. } & 
{In summary, the future of \textit{quantum entanglement} in computing and AI is still uncertain with numerous unresolved issues. These include developing stable, practical quantum computers, creating quantum algorithms applicable to a broad range of problems, and successfully integrating quantum computing into classical systems and AI. It is crucial not to overlook the vast scientific and practical challenges that precede it. }
\\ \hline
\bottomrule
\end{tabular}
\end{small}
\caption{Debate subject: \textit{Quantum entanglement} holds tremendous potential to revolutionize computing and advance artificial intelligence?}
\label{tab:Quantum-Debate}
\end{table*}

\begin{figure}[ht!]
  \centering
  \includegraphics[width=1.0\linewidth]{Chapter6/Table6.6.4.png}
  \vspace{-.03in}
\caption{Debate subject: \textit{Quantum entanglement} holds tremendous potential to revolutionize computing and advance artificial intelligence?}
\label{tab:Quantum-Debate}
  \vspace{-.1in}
\end{figure}
\end{comment}


\begin{comment}
\section*{Appendix D: Content Quality Evaluation Criteria }

\begin{table*}[th!]
\begin{center}
\begin{small}
\begin{tabular}{|p{0.2\linewidth}|p{0.6\linewidth}|}
\toprule
\hline
\textbf{Criteria} & \textbf{Description} \\ \hline
Well written & Its prose is engaging and of a professional standard. \\ \hline
Comprehensive & It neglects no major facts or details and places the subject in context. \\ \hline
Well researched & It is a thorough and representative survey of the relevant literature; claims are verifiable against high-quality reliable sources and are supported by inline citations where appropriate. \\ \hline
Neutral & It presents views fairly and without bias. \\ \hline
Stable & It is not subject to ongoing edit wars and its content does not change significantly from day to day, except in response to the featured article process. \\ \hline
Copyright compliant & Compliant with Wikipedia's copyright policy and free of plagiarism or too-close paraphrasing. \\ \hline
Lead section & It has a concise lead section that summarizes the topic and prepares the reader for the detail in the subsequent sections. \\ \hline
Verifiable & Information on Wikipedia must be verifiable; if no reliable third-party sources can be found on a topic, then it should not be included in Wikipedia. \\ \hline
Consistent citations & Consistently formatted inline citations using footnotes where required by criterion 1c, with suggestions on formatting references found in citing sources. \\ \hline
Media & It includes images and other media, where appropriate, with succinct captions and acceptable copyright status. \\ \hline
Length & It stays focused on the main topic without going into unnecessary detail and uses summary style where appropriate. \\ \hline
No original research & all material in Wikipedia must be attributable to a reliable, published source. \\ \hline
No promotion & {Articles should not serve as promotional material or advertisements.} \\ \hline 
\bottomrule
\end{tabular}
\end{small}
\end{center}
\caption{Criteria for a Well-Rated Wikipedia Article}
\label{tab:Q_criteria}
\end{table*}

Table~\ref{tab:Q_criteria} lists the criteria of Wikipedia's editorial board for assessing content quality.
    
\end{comment}
