# Supplementary material for: Unlocking the Wisdom of Large Language Models: An Introduction to The Path to Artificial General Intelligence
Source: arXiv:2409.01007 source file (2025-04-15)
Supplement: Supplementary file 17 [file AppendixZ.tex]

\section*{Appendix A: Experiment \#1 Justifications of 31 Biased Articles}

In Chapter~\ref{sec:exp1}, we note that $\EVINCE$ processed 31 news articles to assess their neutrality. In addition to the final decision, we detail the justifications $\EVINCE$ provides at the debate's end.  These
justifications are documented in four tables: Tables~\ref{tab:Z11}, \ref{tab:Z12}, \ref{tab:Z21}, and \ref{tab:Z22}.

\begin{comment}
Figure~\ref{fig:D-biases} depicts
the voting distances between S ($\EVINCE$), D (Democrat), and R (Republican).
S is centric compared with D and R.
We have also discussed in the main body of the paper that D tends to defend D's
scandals and R defends R's. This shows
a problem on relying humans to annotate
sensitive data, where 
personal demographics and emotion
may lead to biased annotations and
inaccurate ground truths.

\begin{figure*}[th!]
\vspace{-.1in}
\begin{center}
\includegraphics[width=0.90\linewidth]{Biases-D-Scandals.png} \\
\vspace{-.3in}
\includegraphics[width=0.98\linewidth]{Biases-R-Scandals.png}
\end{center}
\vspace{-.3in}
\caption{Distances between S, D, and R's Bias Ratings 
on Democrat \& Republican scandals.}
\label{fig:D-biases}
\vspace{-.2in}
\end{figure*}
\end{comment}

\begin{table}[thb!]
\vspace{-.05in}
\centering
\begin{scriptsize}
%\begin{tabular}{|l|l|l|}
\begin{tabular}{|p{0.045\linewidth}|p{0.08\linewidth}|p{0.78\linewidth}|}
\toprule
\hline
{\#} & {Rating \par S,{\color{blue}D},{\color{red}R}} & {$\EVINCE$ Justifications}  
\\ \hline
{D1} &
{5,{\color{blue}5},{\color{red}5}} & 
{The article discusses the controversy surrounding the IRS’s alleged targeting of conservative groups, focusing on Rep. Darrell Issa’s stance against releasing full transcripts from IRS interviews. Issa argues that full disclosure would compromise the investigation, a position criticized by Rep. Elijah Cummings, who advocates for transparency. The debate highlights political tensions, with implications of bias in the handling of the investigation. The article portrays a complex interplay of political, ideological, and possibly historical biases, reflecting the contentious nature of the IRS scandal and its investigation.}  \\ \hline
{D2} & 
{5,{\color{blue}5},{\color{red}3}} & 
The article discusses Michele Bachmann’s statement that the IRS scandal, involving the targeting of conservative groups, undermines the credibility of the 2012 election. Bachmann accuses the Obama administration of lying and questions the impartiality of the IRS, particularly in relation to health care coverage for conservatives. The article reflects political and ideological biases, given its focus on Bachmann’s perspective and the implications for the election’s integrity and government trustworthiness.

The perception of bias in Michele Bachmann’s statement about the IRS scandal primarily stems from the framing and implications of her comments. She directly links the IRS’s actions to the credibility of the 2012 election and the Obama administration, suggesting a deliberate misuse of power for political gain. This perspective inherently carries ideological and political biases by casting the issue in a light that emphasizes misconduct by one political group over another, without presenting counterarguments or broader context that might mitigate or challenge that viewpoint.
\\ \hline
{D8} & 
{3,{\color{blue}5},{\color{red}2}} & 
The reporting appears to maintain a neutral tone by directly stating the facts and comments made by John Kerry and others involved without inserting opinionated language. It discusses the global reaction to the NSA's surveillance practices and includes Kerry's acknowledgment of overreach, as well as the international and domestic fallout from these revelations. The inclusion of various perspectives, including those from technology companies and international officials, alongside Kerry's comments, aims to provide a balanced view of the situation.
\\ \hline
{D31} & 
{3,{\color{blue}5},{\color{red}3}} &
{The CNN article appears to report on Ray Nagin's indictment with a focus on the factual and legal aspects of the case, without displaying overt biases related to politics, ideology, religion, gender, race, socioeconomic status, culture, geography, or history. By sticking closely to the details of the indictment and Nagin's public actions and statements, the article provides a comprehensive overview of the charges against him while maintaining journalistic neutrality.}
\\ \hline
\bottomrule
\end{tabular}
\end{scriptsize}
\vspace{-.08in}
\caption{The First 9 of 16 Democrat Scandals News Articles
Rated by $\EVINCE$ and its Justifications.  The rating column
starts with $\EVINCE$'s rating, the Democrat rater (in {\color{blue}blue}), and
then Republican rater (in {\color{red}red}).}
\label{tab:Z11}
\end{table}

\begin{table*}[th!]
\vspace{.05in}
\centering
\begin{scriptsize}
%\begin{tabular}{|l|l|l|}
\begin{tabular}{|p{0.045\linewidth}|p{0.08\linewidth}|p{0.78\linewidth}|}
\toprule
\hline
{D106} & 
{3,{\color{blue}3},{\color{red}3}} &
The article reports on former Detroit Mayor Kwame Kilpatrick's sentencing to 28 years in prison for public corruption, emphasizing the gravity of his crimes against the city's welfare. It contrasts Kilpatrick's actions with the impact on Detroit, highlighting the judicial and public response to his extensive criminal activities. The reporting focuses on factual recounting of the trial's outcome, Kilpatrick's and his co-defendant's crimes, and the broader implications for Detroit, without evident bias towards political, ideological, or other specific perspectives.
\\ \hline
{D109} & 
{4,{\color{blue}4},{\color{red}3}} &
The article's bias primarily stems from its focus on internal Democratic opposition to Lawrence Summers' Federal Reserve Chair nomination, highlighting a lack of unity and strategy within the party and the White House's mismanagement of the nomination process. It suggests an underestimation of the opposition's seriousness by the White House, portraying the administration in a somewhat negative light for not engaging more proactively with concerned Senate Democrats.
\\ \hline
{D157} & 
{4,{\color{blue}4},{\color{red}3}} &
The article discusses the challenges in U.S.-Germany intelligence relations following revelations of U.S. surveillance on Chancellor Merkel. Despite efforts to rebuild trust, significant differences in surveillance philosophies persist, with the U.S. prioritizing security interests and Germany emphasizing privacy and alliance values. The situation reflects broader tensions in U.S. relations with allies over privacy and surveillance practices.

The article's framing might suggest a bias towards highlighting the challenges and frictions in the U.S.-Germany intelligence relations, particularly emphasizing Germany's privacy concerns and skepticism towards U.S. surveillance practices. It portrays the U.S. stance as unyielding and contrasts this with Germany's emphasis on privacy and legal constraints, potentially casting the U.S. in a more negative light regarding international surveillance and cooperation.
\\ \hline
{D188} & 
{4,{\color{blue}3},{\color{red}3}} &
The article reports that Hillary Clinton received warnings about security threats in Benghazi before the 2012 attack through emails. These were part of around 300 emails released by the State Department, which also show Clinton's responses and thoughts during the aftermath. The political controversy regarding the Obama administration's initial assessment of the attack's cause is also mentioned, with references to Susan Rice's statements on talk shows.

The reporting may exhibit bias through selective emphasis on Clinton's receipt of warnings about security threats in Benghazi and her responses, potentially framing her actions or inactions in a negative light. The focus on the political controversy and the administration's initial assessment of the attack's cause could also influence perceptions of responsibility or competence.
\\ \hline
\bottomrule
\end{tabular}
\end{scriptsize}
\vspace{.08in}
\caption{The Last 7 of 16 Democrat Scandals News Articles
Rated by $\EVINCE$ and its Justifications.  The rating column
starts with $\EVINCE$'s rating, the Democrat rater (in {\color{blue}blue}), and
then Republican rater (in {\color{red}red}).}
\vspace{.18in}
\label{tab:Z12}
\end{table*}

\begin{table*}[th!]
\vspace{.05in}
\centering
\begin{scriptsize}
%\begin{tabular}{|l|l|l|}
\begin{tabular}{|p{0.045\linewidth}|p{0.08\linewidth}|p{0.78\linewidth}|}
\toprule
\hline
{\#} & {Rating \par S,{\color{blue}D},{\color{red}R}} & {$\EVINCE$ Justifications}  
\\ \hline
{R1} &
{5,{\color{blue}3},{\color{red}5}} & 
{The editorial from The New York Times Editorial Board exhibits a clear bias against the Republican party's handling of the Benghazi attack investigation, framing it as politically motivated rather than a genuine effort to address security failures or seek accountability. The language and tone used in the editorial are critical and dismissive of the Republicans' actions, suggesting a political and ideological bias. While editorials are inherently opinion-based and are expected to take a stance, this piece clearly communicates a stance that is critical of the Republicans' focus on Benghazi, suggesting a lack of neutrality in its assessment of the motives and actions surrounding the investigation.}  \\ \hline
{R7} & 
{3,{\color{blue}3},{\color{red}3}} & 
The article reports on allegations by Senator Mitch McConnell that his campaign headquarters were wiretapped, with the FBI investigating these claims. A recording of McConnell's team discussing potential attacks on Ashley Judd, who was considering running against him, was released by Mother Jones. McConnell accused the political left of this action, describing it as a "Nixonian move." The recording included discussions on various strategies to undermine potential opponents, highlighting a focus on Judd's personal struggles and political views. The controversy has prompted responses from both Republican and Democratic officials, reflecting the tense political atmosphere.
\\ \hline
{R69} & 
{4,{\color{blue}4},{\color{red}4}} &
{The report discusses how young Republicans are seeking a different message for  elections, emphasizing a departure from divisive social issues and a focus on fiscal responsibility, national defense, and energy advancement. 

Selection Bias: The article primarily focuses on young Republicans who are seeking a different message for the party. It doesn't provide as much insight into young Republicans who may still align with traditional conservative values, which could create a slight bias toward the viewpoints of those seeking change.

Language Bias: Certain language choices, such as describing divisive social issues as "anti-abortion, anti-gay, and anti-environment stances," may reflect a bias toward more progressive viewpoints on these issues. A more neutral description might be "positions on abortion, same-sex marriage, and environmental policy."

Source Bias: The perspectives provided in the article are mainly from young Republicans themselves. While including these voices is essential, the article could benefit from additional perspectives from political analysts or experts to provide more context and balance.
}
\\ \hline
\bottomrule
\end{tabular}
\end{scriptsize}
\vspace{.08in}
\caption{The First 8 of 15 Republican Scandals News Articles
Rated by $\EVINCE$ and its Justifications.  The rating column
starts with $\EVINCE$'s rating, the Democrat rater (in {\color{blue}blue}), and
then Republican rater (in {\color{red}red}).}
\label{tab:Z21}
\end{table*}

\begin{table*}[th!]
\vspace{.05in}
\centering
\begin{scriptsize}
%\begin{tabular}{|l|l|l|}
\begin{tabular}{|p{0.045\linewidth}|p{0.08\linewidth}|p{0.78\linewidth}|}
\toprule
\hline
{\#} & {Rating \par S,{\color{blue}D},{\color{red}R}} & {EVINCE Justifications}  
\\ \hline
{R214} & 
{5,{\color{blue}3},{\color{red}5}} &
The Daily Kos article clearly exhibits political and ideological bias, with a tone and language that are critical of the Republicans. It uses the incident involving Dave Agema to argue that the party's efforts to rebrand itself as more tolerant and inclusive are undermined by its members' actions. While the article includes factual information regarding the incident and the party's response, its presentation and commentary are aligned with a progressive viewpoint, aiming to highlight and criticize perceived contradictions and failures within the Republican Party. This approach is consistent with opinion journalism but introduces bias through its critical tone, selective presentation of information, and framing of the incident as emblematic of broader issues within the party.
\\ 
\hline 
{R221} &
{3,{\color{blue}3},{\color{red}4}} & 
{"Hurricane Christie" presents Governor Chris Christie's critique of House Republicans in a manner that emphasizes party conflict and personal betrayal. The dramatic framing, choice of language, and focus on internal discord may introduce bias by portraying Christie's actions in a specific light and emphasizing the divide within the Republican Party. The article's approach to presenting these events can influence readers' perceptions, potentially leading them to see the situation through a lens of heightened drama and internal strife.}  
\\ \hline
{R233} & 
{4,{\color{blue}3},{\color{red}4}} & 
While the article attempts to cover the last-ditch efforts by House Republicans to avert a government shutdown and the standoff with Senate Democrats, the framing and language used may introduce a bias towards portraying the Republican efforts in a more favorable light. By emphasizing the Republican narrative of seeking negotiation and characterizing the Democratic response as dismissive, the article could be perceived as leaning towards a particular political perspective. The inclusion of quotes and perspectives from both sides does provide a degree of balance, but the overall presentation and emphasis could influence readers' perceptions of the shutdown negotiations.
\\ \hline
{R235} & 
{3,{\color{blue}5},{\color{red}5}} & 
Without knowledge of the author or publication, this text attempts to navigate a complex and sensitive story by providing details from multiple sources, including the main figures involved, political watchdog groups, and law enforcement. It balances the serious allegations with responses from the accused, background information, and the current status of investigations. While the focus on unsubstantiated claims could inherently sway public opinion, the article's inclusion of diverse perspectives and context aims to mitigate overt bias.
\\ \hline
\bottomrule
\end{tabular}
\end{scriptsize}
\vspace{.08in}
\caption{The Last 7 of 15 Republican Scandals News Articles
Rated by $\EVINCE$ and its Justifications.  The rating column
starts with $\EVINCE$'s rating, the Democrat rater (in {\color{blue}blue}), and
then Republican rater (in {\color{red}red}).}
\vspace{.08in}
\label{tab:Z22}
\end{table*}
